# Supplementary material for: Bayesian Projection of Life Expectancy Accounting for the HIV/AIDS Epidemic
Source: arXiv:1608.07330 source file (2016-09-27)
Supplement: Supplementary file 1 [file AppendixUNEPPHIVnonART.pdf]

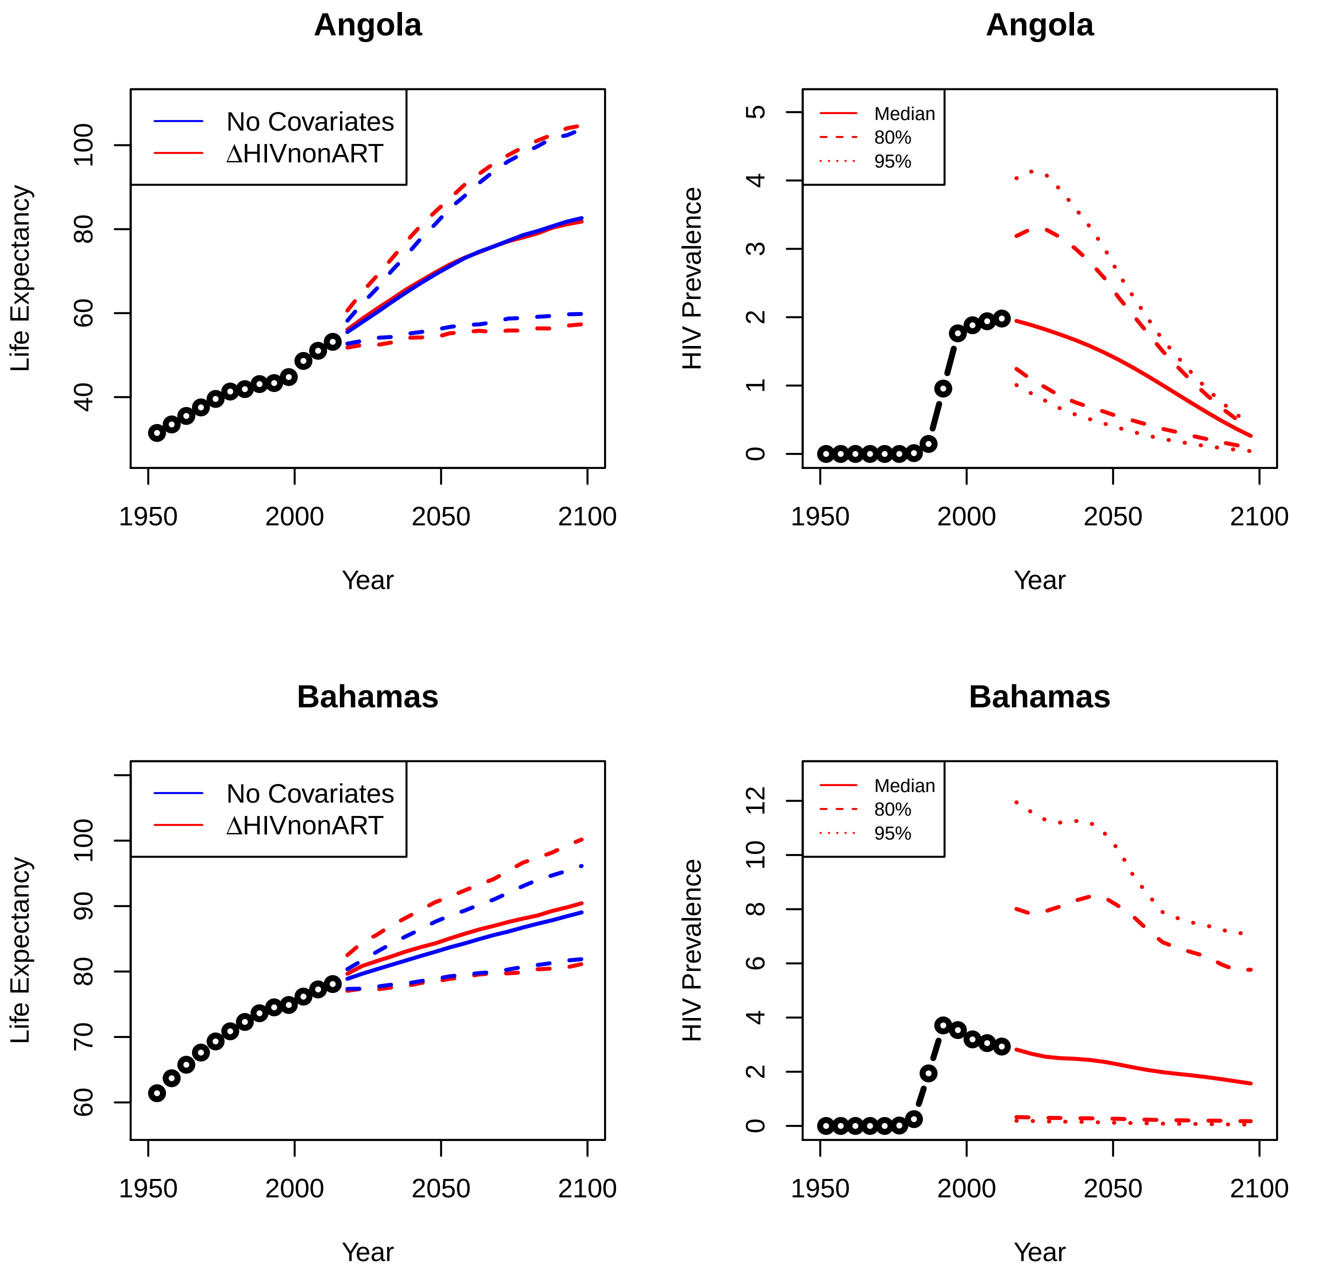
Angola
No Covariates
ΔHIVnonART
Life Expectancy
Year
Angola
Median
80%
95%
HIV Prevalence
Year
Bahamas
No Covariates
ΔHIVnonART
Life Expectancy
Year
Bahamas
Median
80%
95%
HIV Prevalence
Year

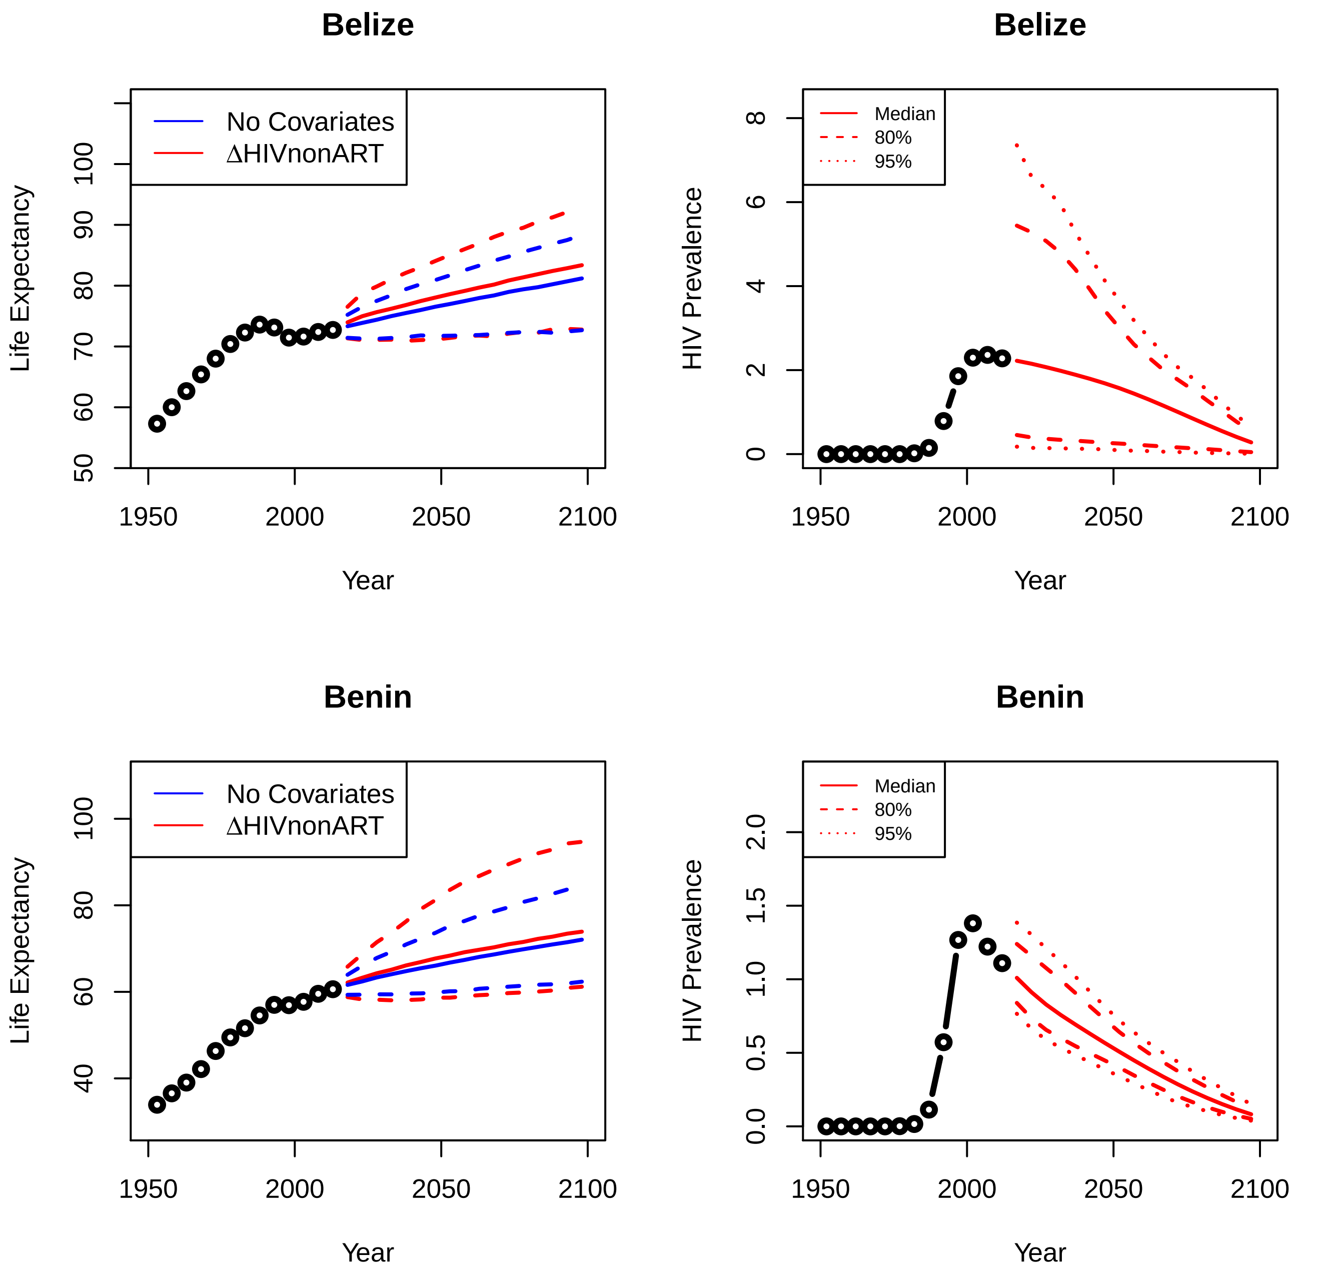
Belize
Life Expectancy
No Covariates
ΔHIVnonART
50
60
70
80
90
100
1950
2000
2050
2100
Year
Belize
HIV Prevalence
Median
80%
95%
0
2
4
6
8
1950
2000
2050
2100
Year
Benin
Life Expectancy
No Covariates
ΔHIVnonART
40
60
80
100
1950
2000
2050
2100
Year
Benin
HIV Prevalence
Median
80%
95%
0.0
0.5
1.0
1.5
2.0
1950
2000
2050
2100
Year

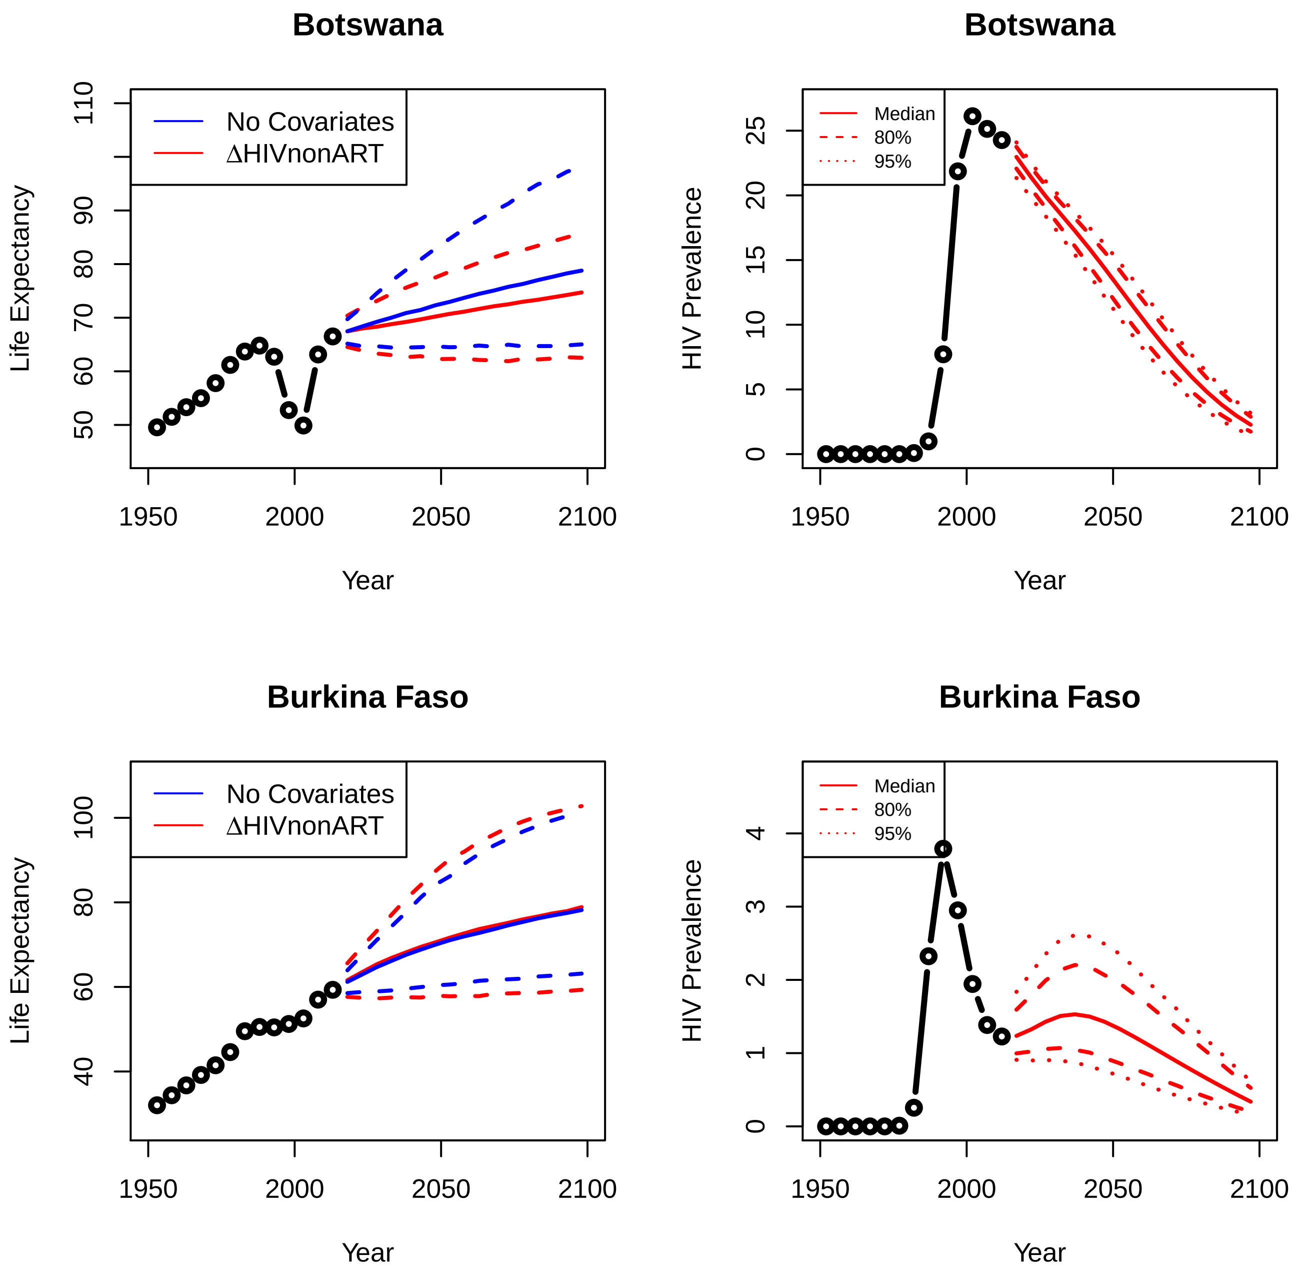

Botswana
No Covariates
ΔHIVnonART
Life Expectancy
50
60
70
80
90
110
1950
2000
2050
2100
Year
Botswana
Median
80%
95%
HIV Prevalence
0
5
10
15
20
25
1950
2000
2050
2100
Year
Burkina Faso
No Covariates
ΔHIVnonART
Life Expectancy
40
60
80
100
1950
2000
2050
2100
Year
Burkina Faso
Median
80%
95%
HIV Prevalence
0
1
2
3
4
1950
2000
2050
2100
Year

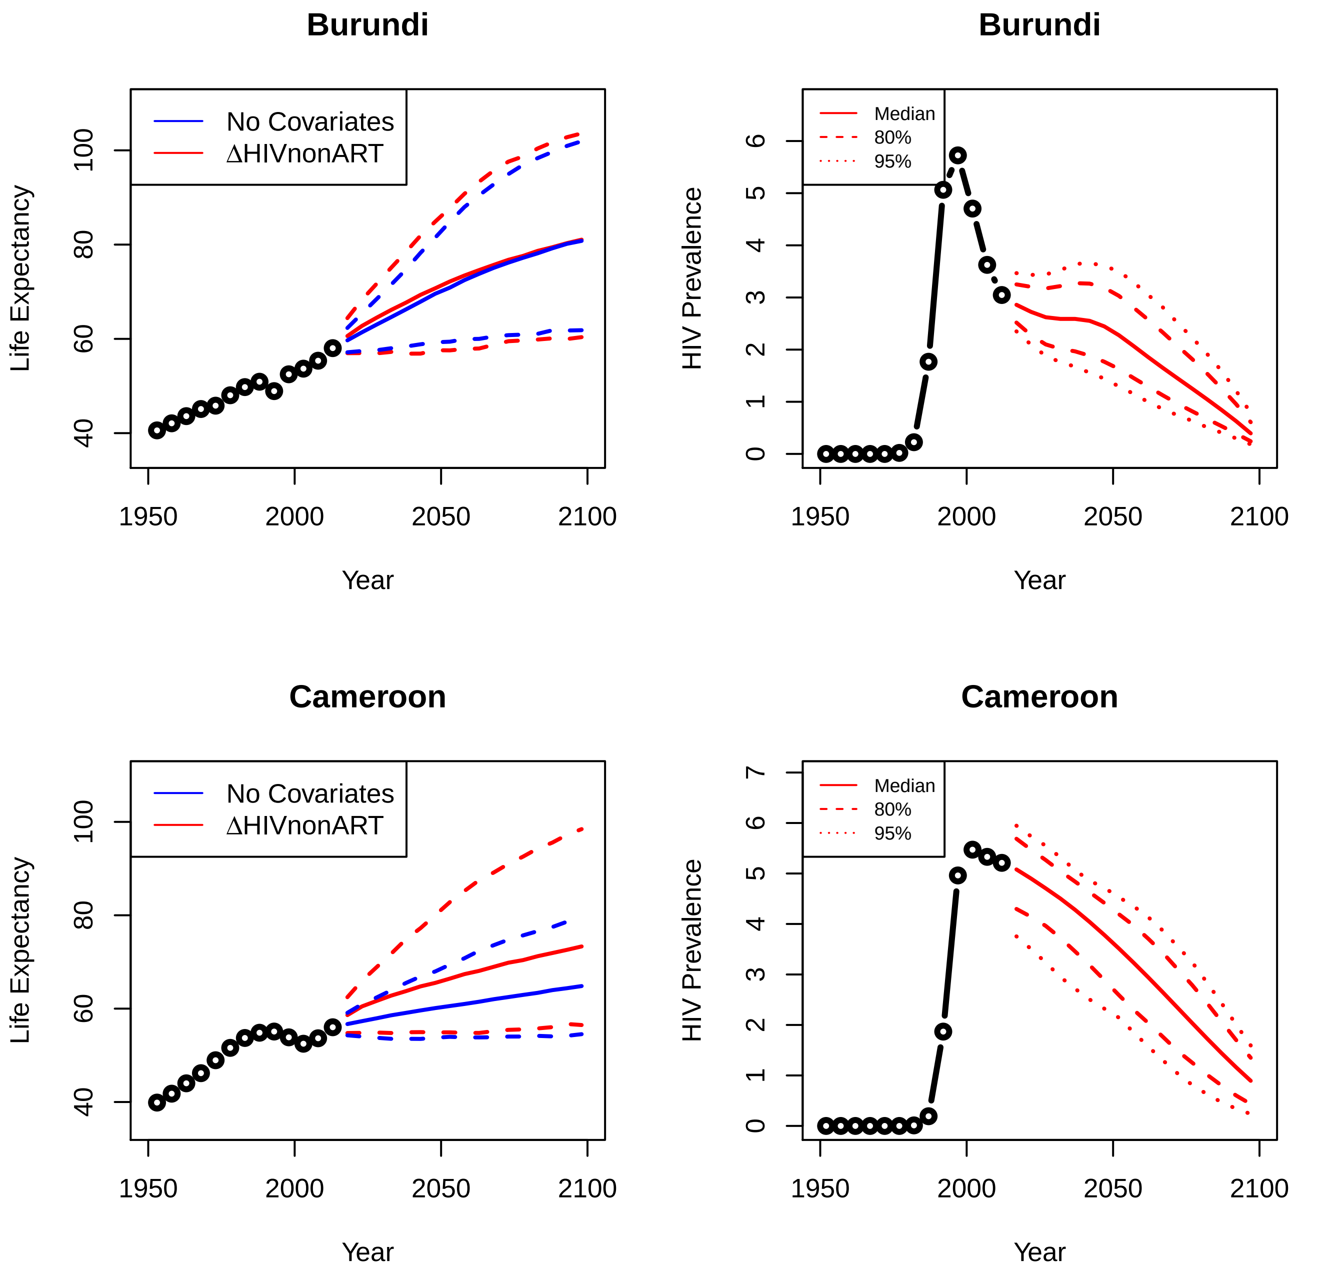

Burundi
No Covariates
ΔHIVnonART
Life Expectancy
40
60
80
100
1950
2000
2050
2100
Year
Burundi
Median
80%
95%
HIV Prevalence
0
1
2
3
4
5
6
1950
2000
2050
2100
Year
Cameroon
No Covariates
ΔHIVnonART
Life Expectancy
40
60
80
100
1950
2000
2050
2100
Year
Cameroon
Median
80%
95%
HIV Prevalence
0
1
2
3
4
5
6
7
1950
2000
2050
2100
Year

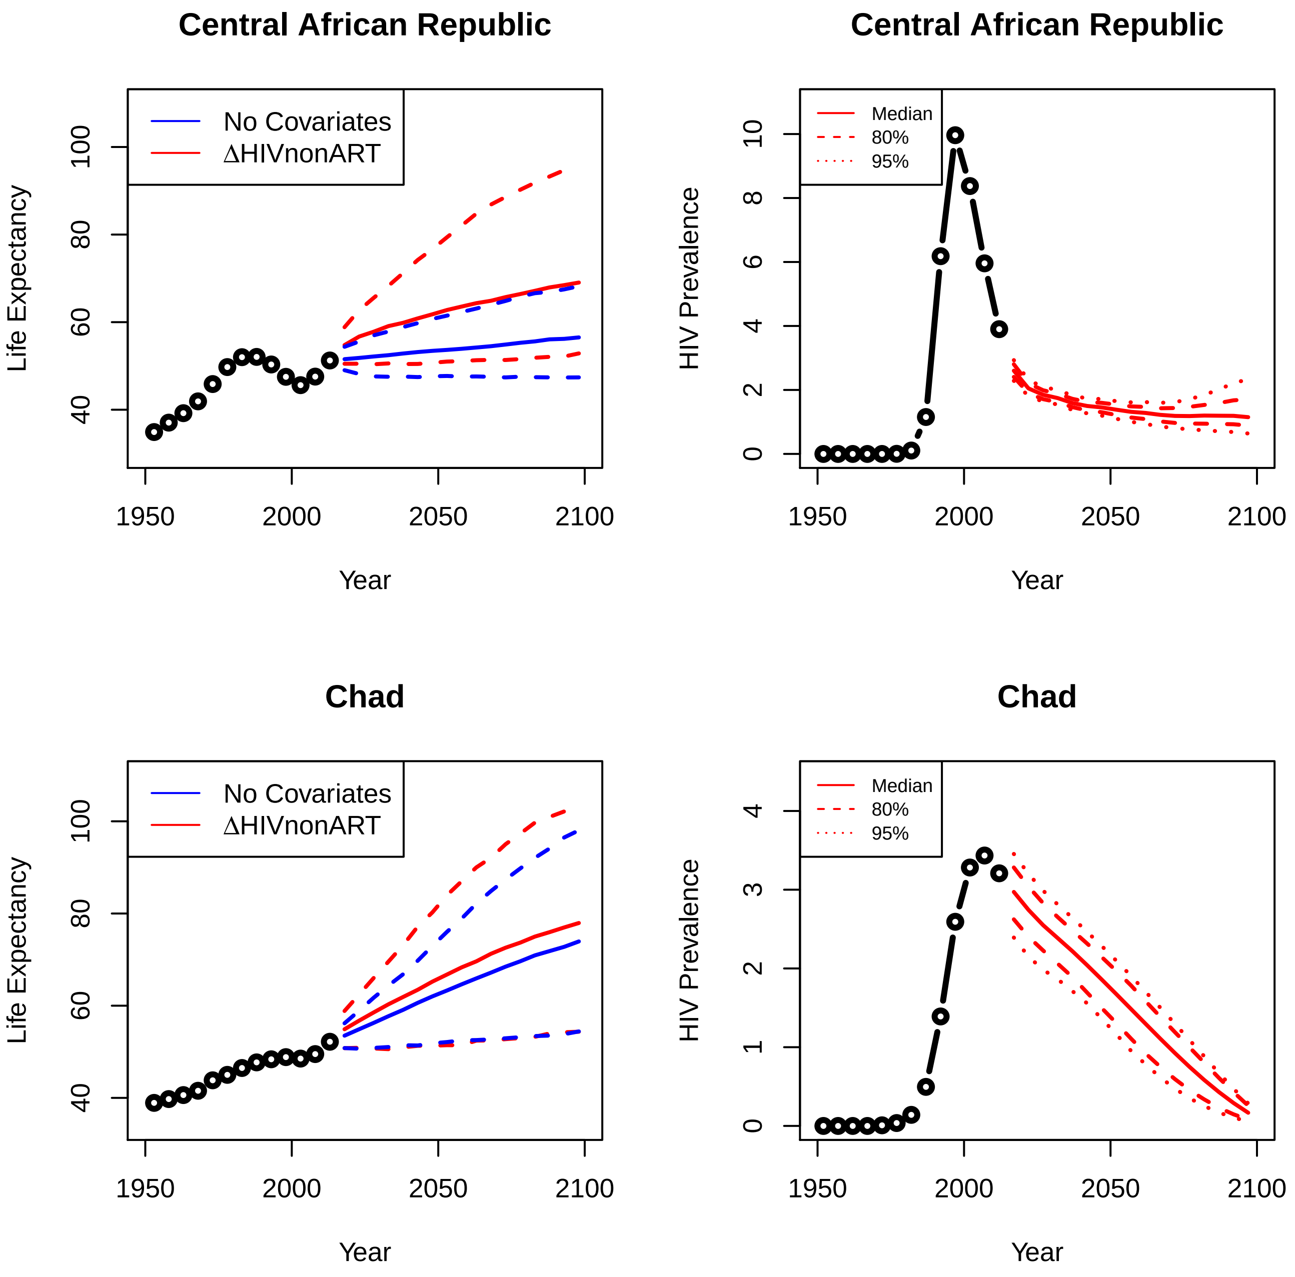
Central African Republic
No Covariates
ΔHIVnonART
Life Expectancy
Year
Central African Republic
Median
80%
95%
HIV Prevalence
Year
Chad
No Covariates
ΔHIVnonART
Life Expectancy
Year
Chad
Median
80%
95%
HIV Prevalence
Year

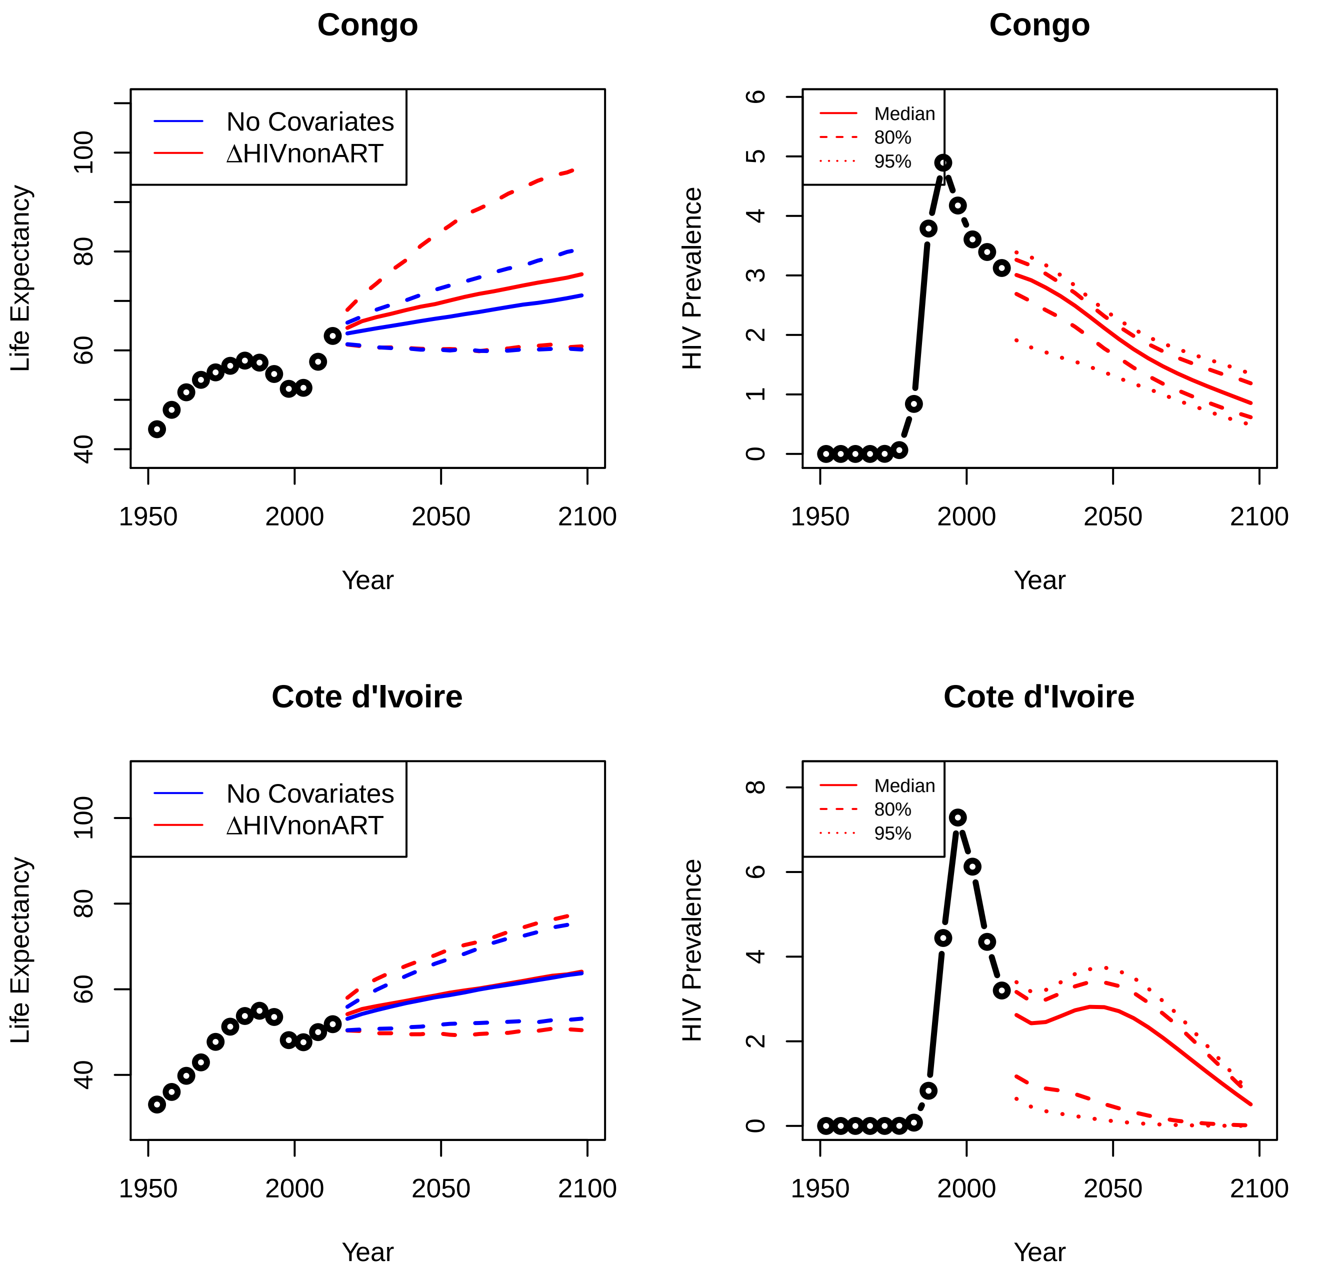

Congo
No Covariates
ΔHIVnonART
Life Expectancy
Year
1950
2000
2050
2100
40
60
80
100
Congo
Median
80%
95%
HIV Prevalence
Year
0
1
2
3
4
5
6
Cote d'Ivoire
No Covariates
ΔHIVnonART
Life Expectancy
Year
Cote d'Ivoire
Median
80%
95%
HIV Prevalence
Year
0
2
4
6
8

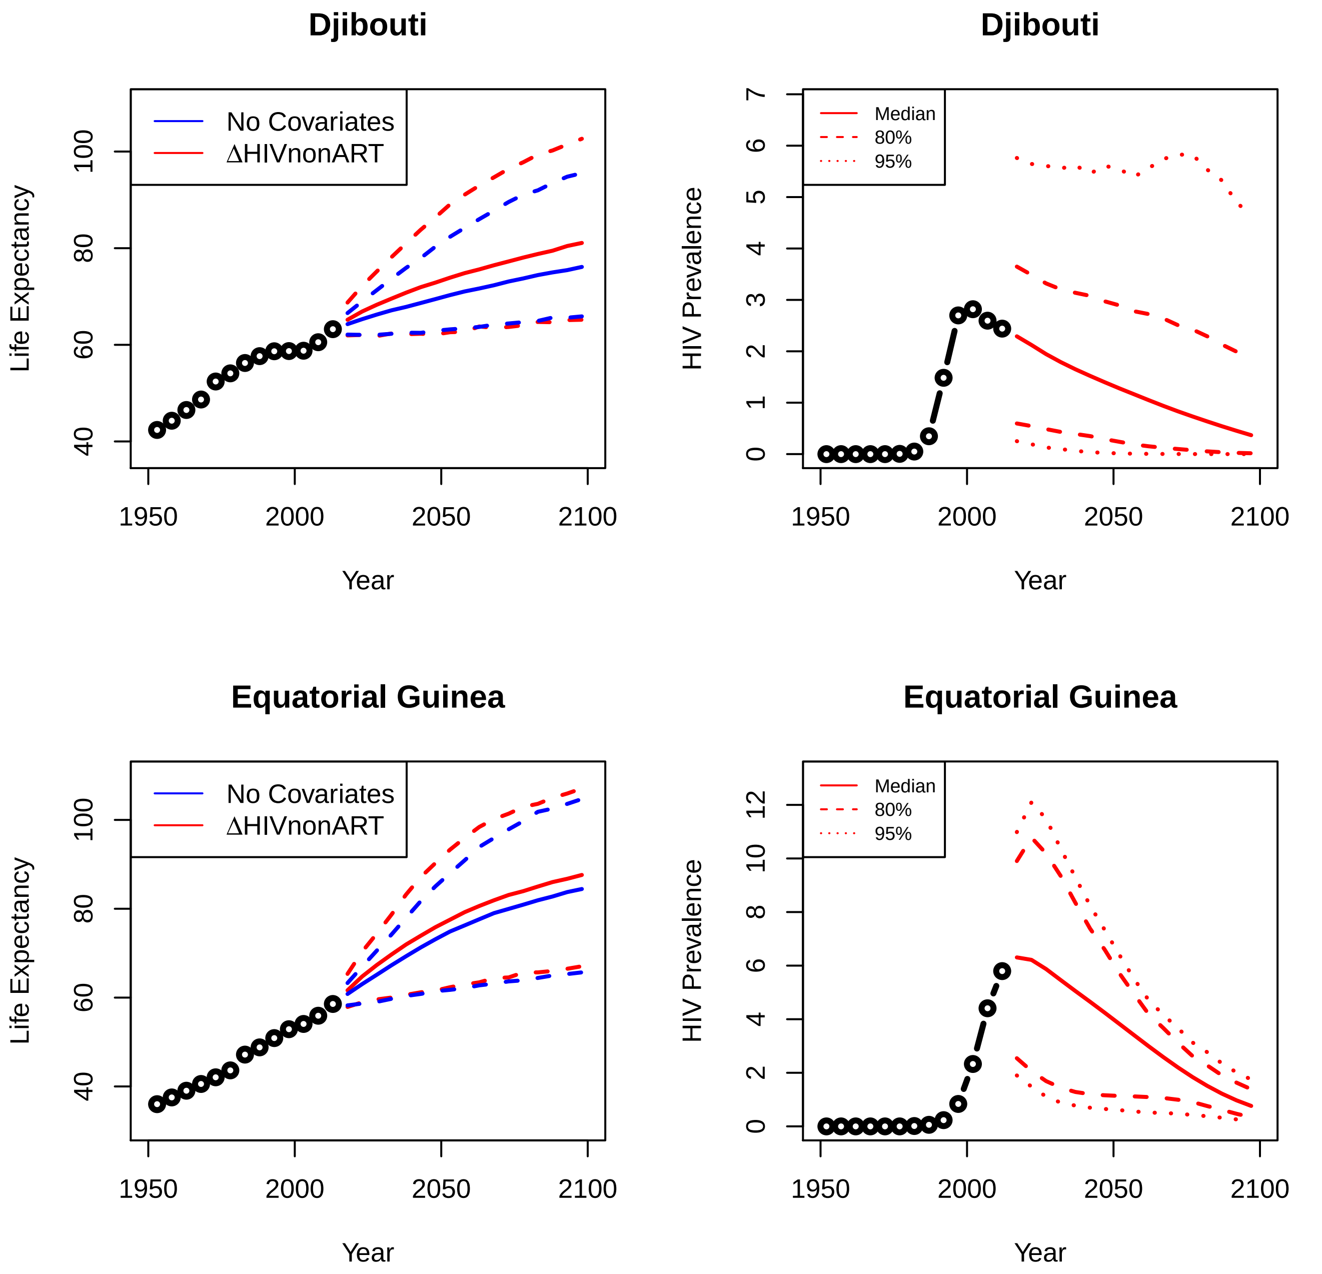
Djibouti
Life Expectancy
Year
No Covariates
ΔHIVnonART
Djibouti
HIV Prevalence
Year
Median
80%
95%
Equatorial Guinea
Life Expectancy
Year
No Covariates
ΔHIVnonART
Equatorial Guinea
HIV Prevalence
Year
Median
80%
95%

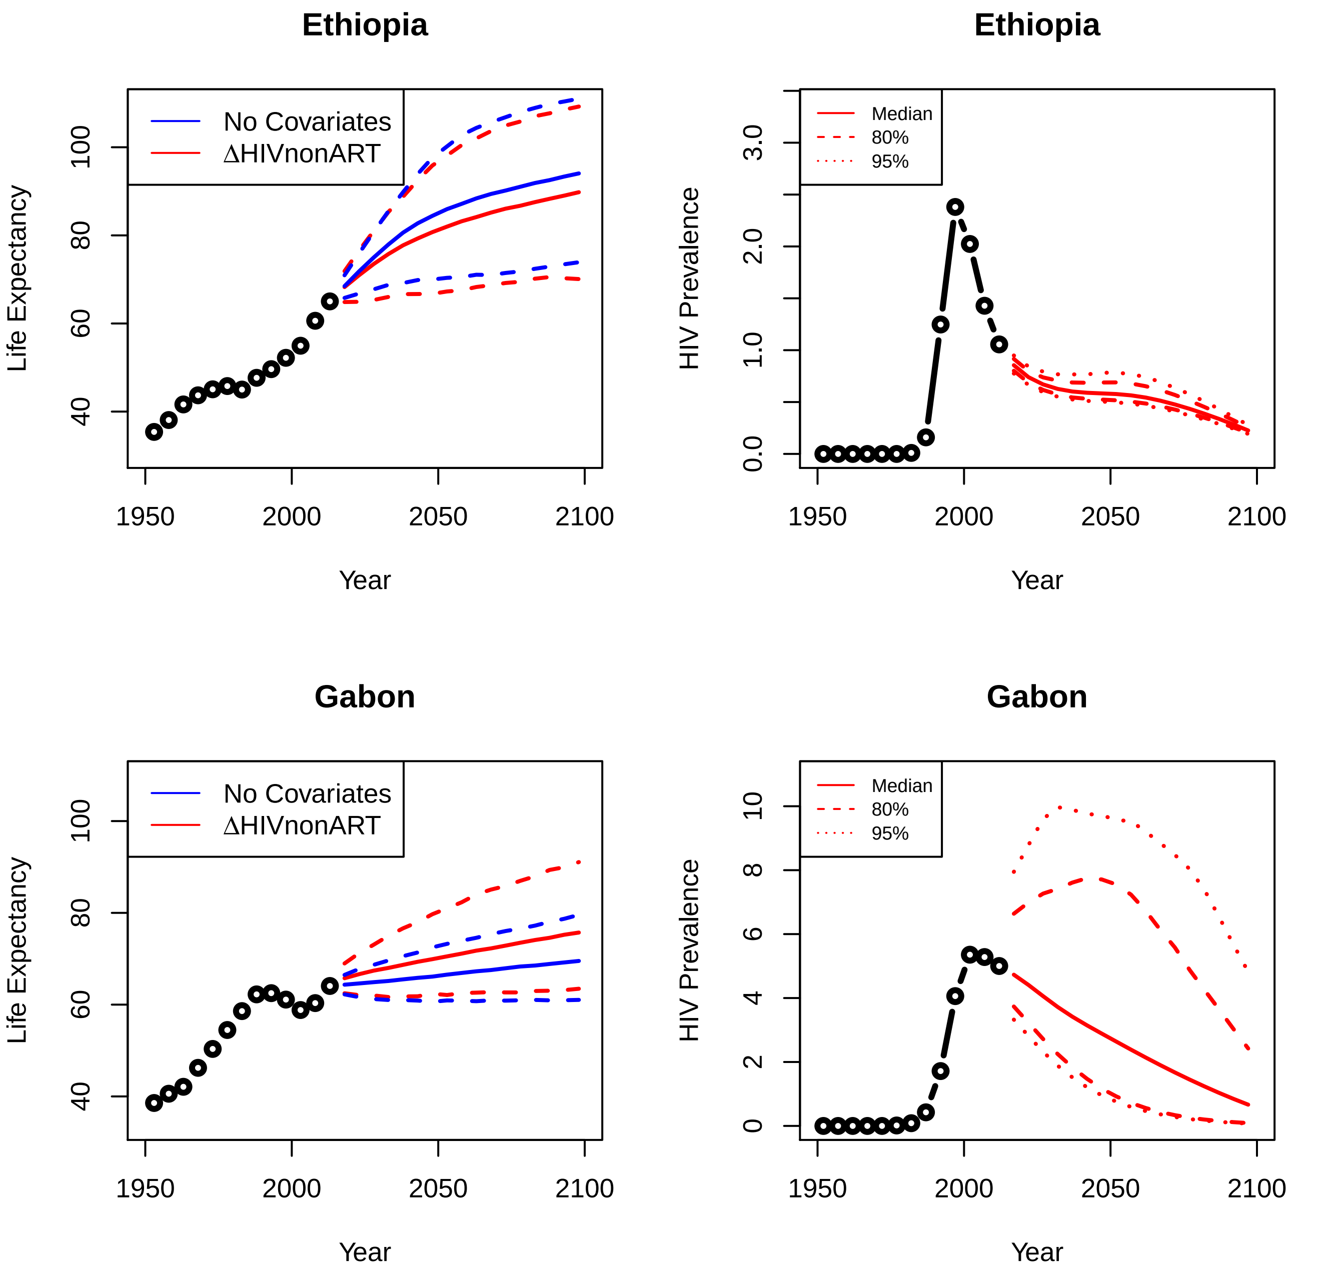
Ethiopia
No Covariates
ΔHIVnonART
Life Expectancy
40
60
80
100
1950
2000
2050
2100
Year
Ethiopia
Median
80%
95%
HIV Prevalence
0.0
1.0
2.0
3.0
1950
2000
2050
2100
Year
Gabon
No Covariates
ΔHIVnonART
Life Expectancy
40
60
80
100
1950
2000
2050
2100
Year
Gabon
Median
80%
95%
HIV Prevalence
0
2
4
6
8
10
1950
2000
2050
2100
Year

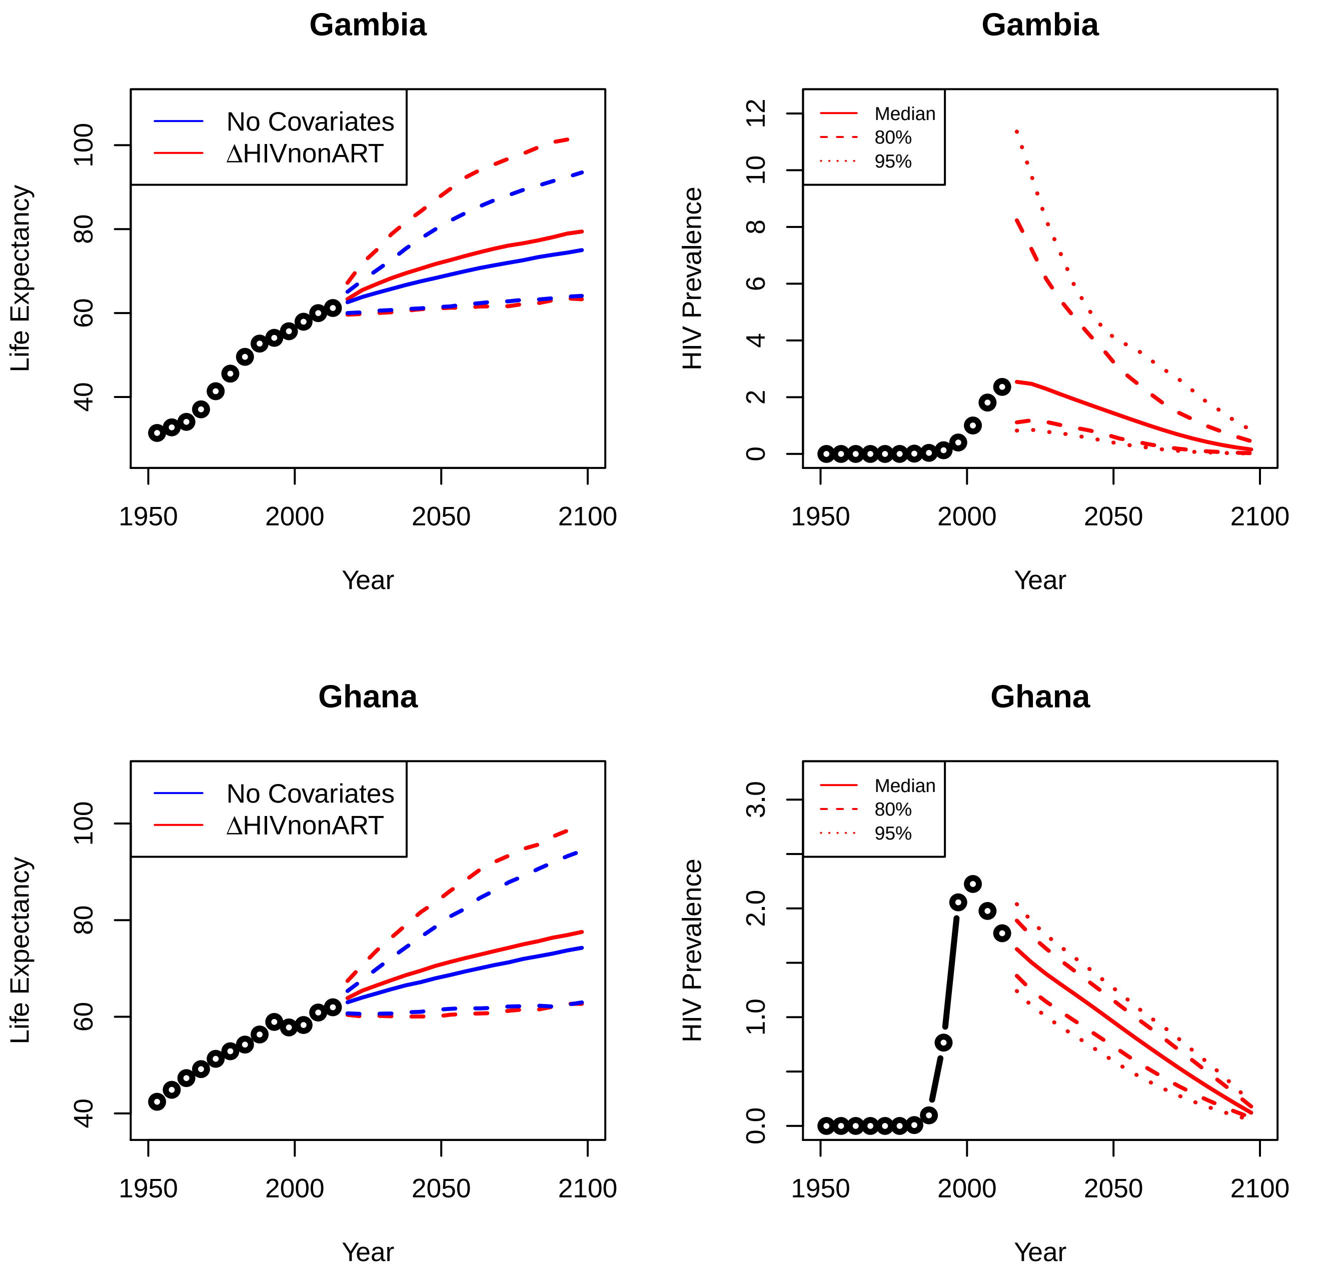
Gambia
No Covariates
ΔHIVnonART
Life Expectancy
Year
Gambia
Median
80%
95%
HIV Prevalence
Year
Ghana
No Covariates
ΔHIVnonART
Life Expectancy
Year
Ghana
Median
80%
95%
HIV Prevalence
Year

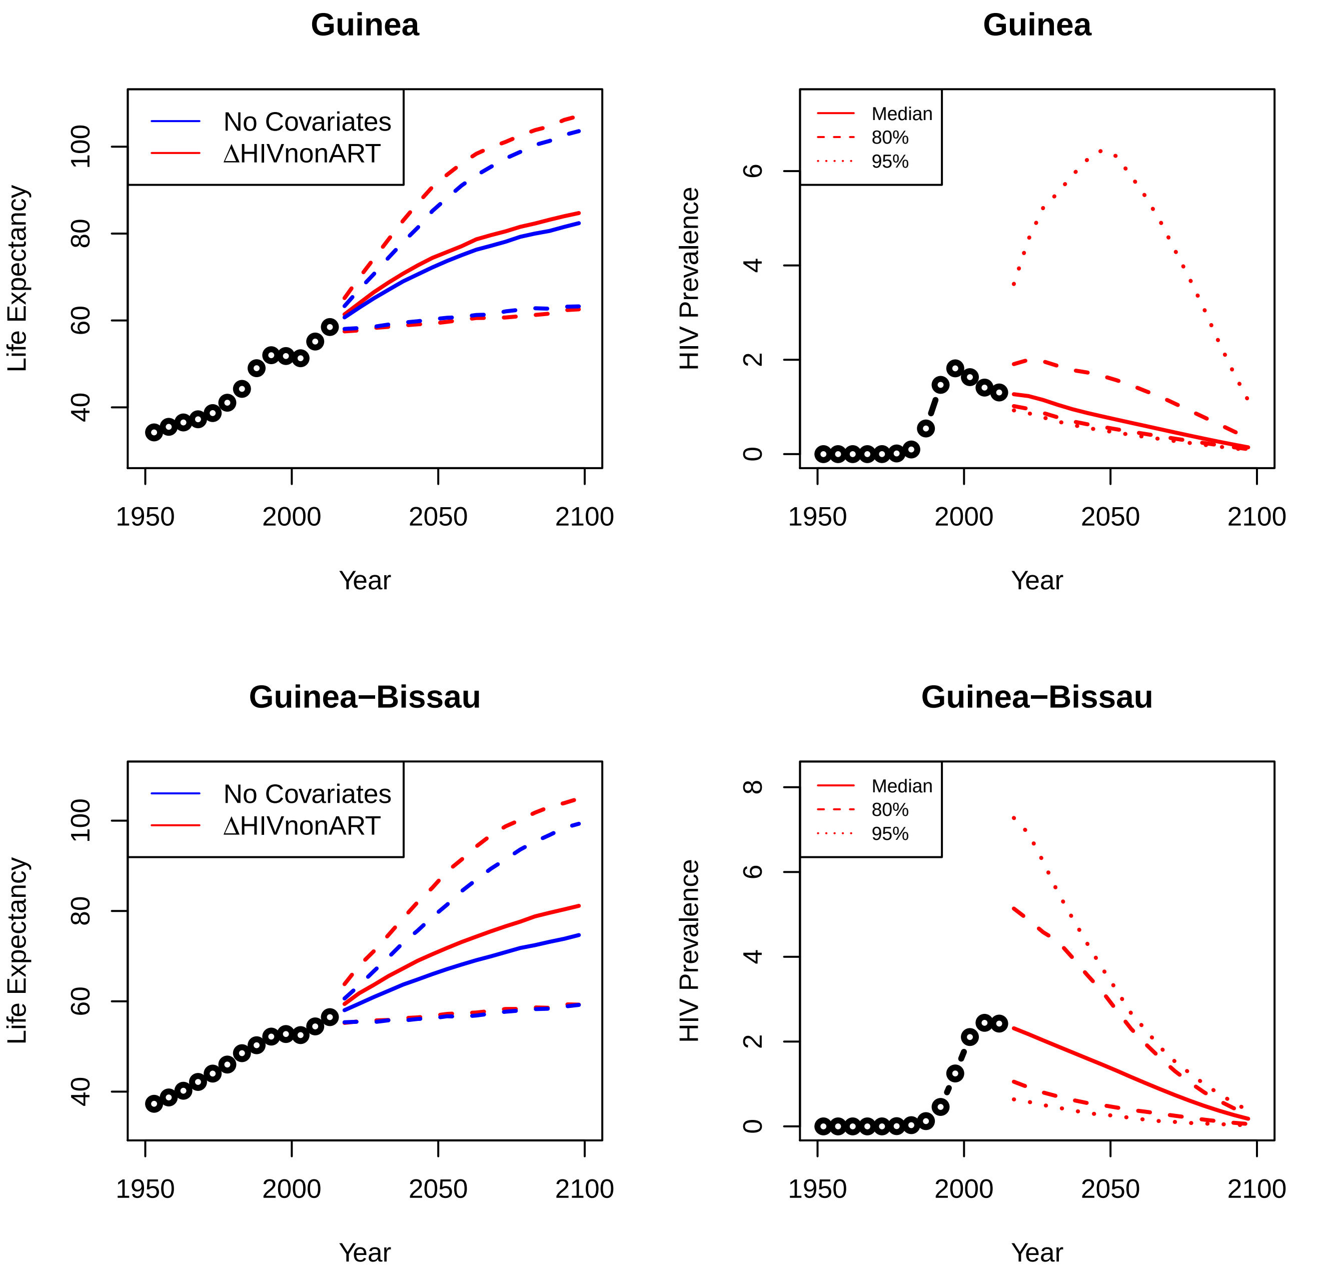
Guinea
No Covariates
ΔHIVnonART
Life Expectancy
Year
Guinea
Median
80%
95%
HIV Prevalence
Year
Guinea−Bissau
No Covariates
ΔHIVnonART
Life Expectancy
Year
Guinea−Bissau
Median
80%
95%
HIV Prevalence
Year

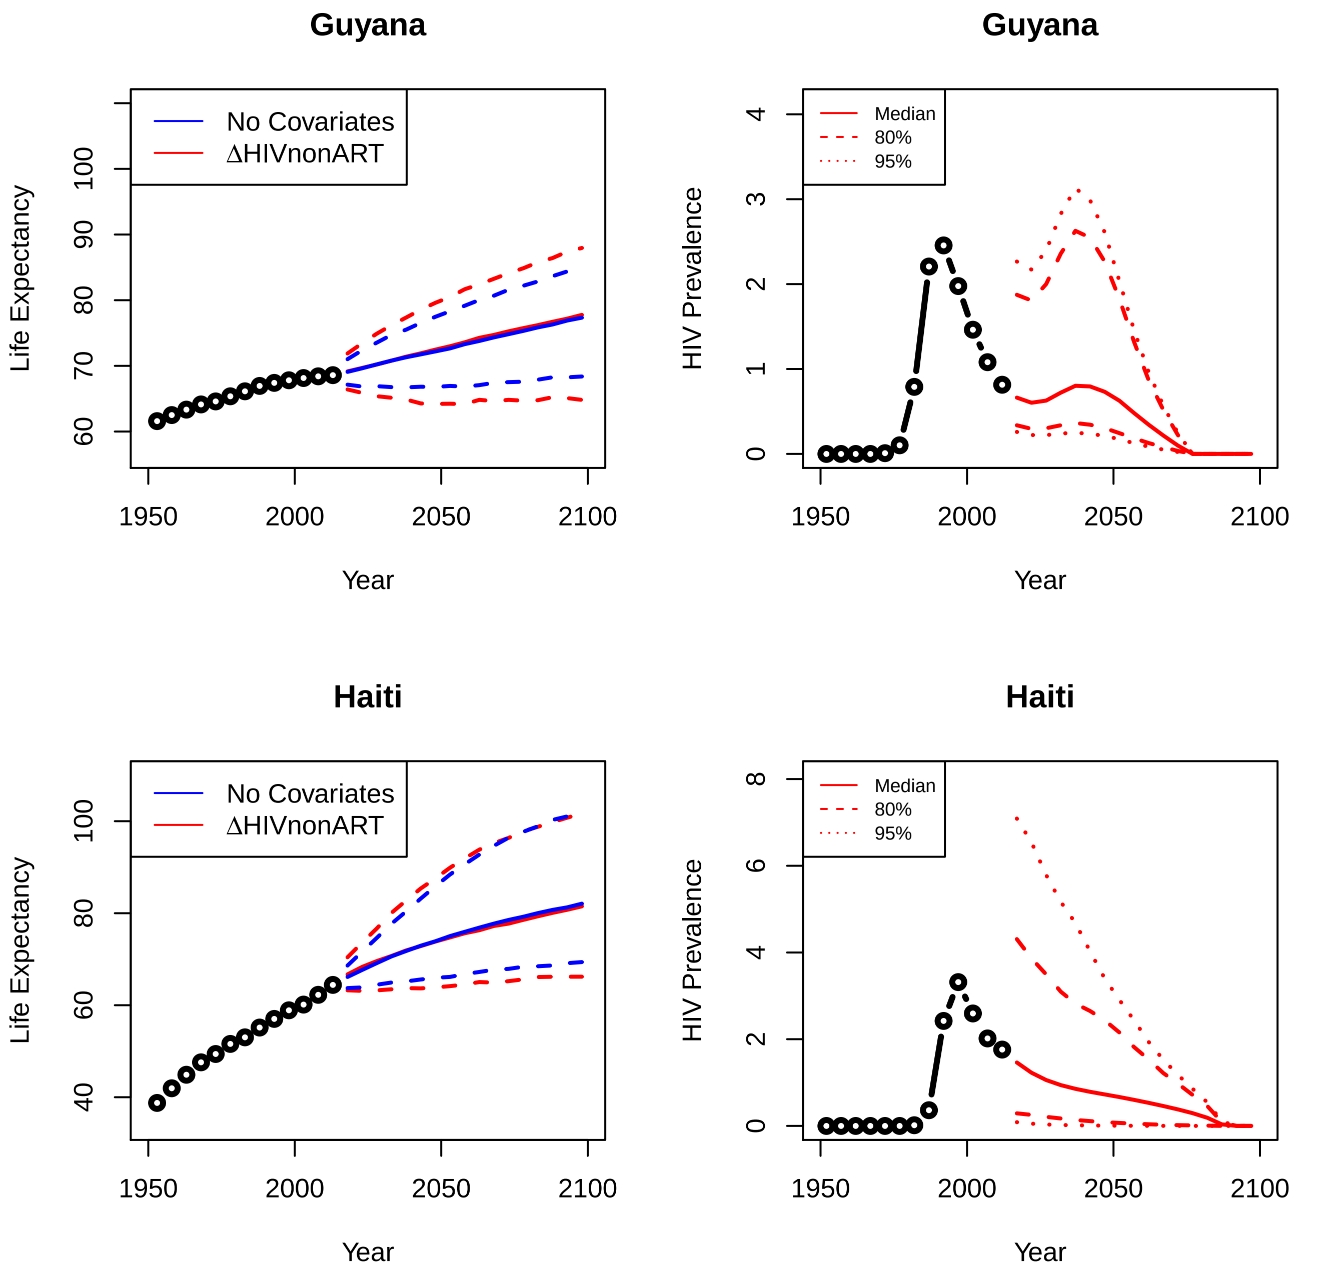

Guyana
No Covariates
ΔHIVnonART
Life Expectancy
Year
Guyana
Median
80%
95%
HIV Prevalence
Year
Haiti
No Covariates
ΔHIVnonART
Life Expectancy
Year
Haiti
Median
80%
95%
HIV Prevalence
Year

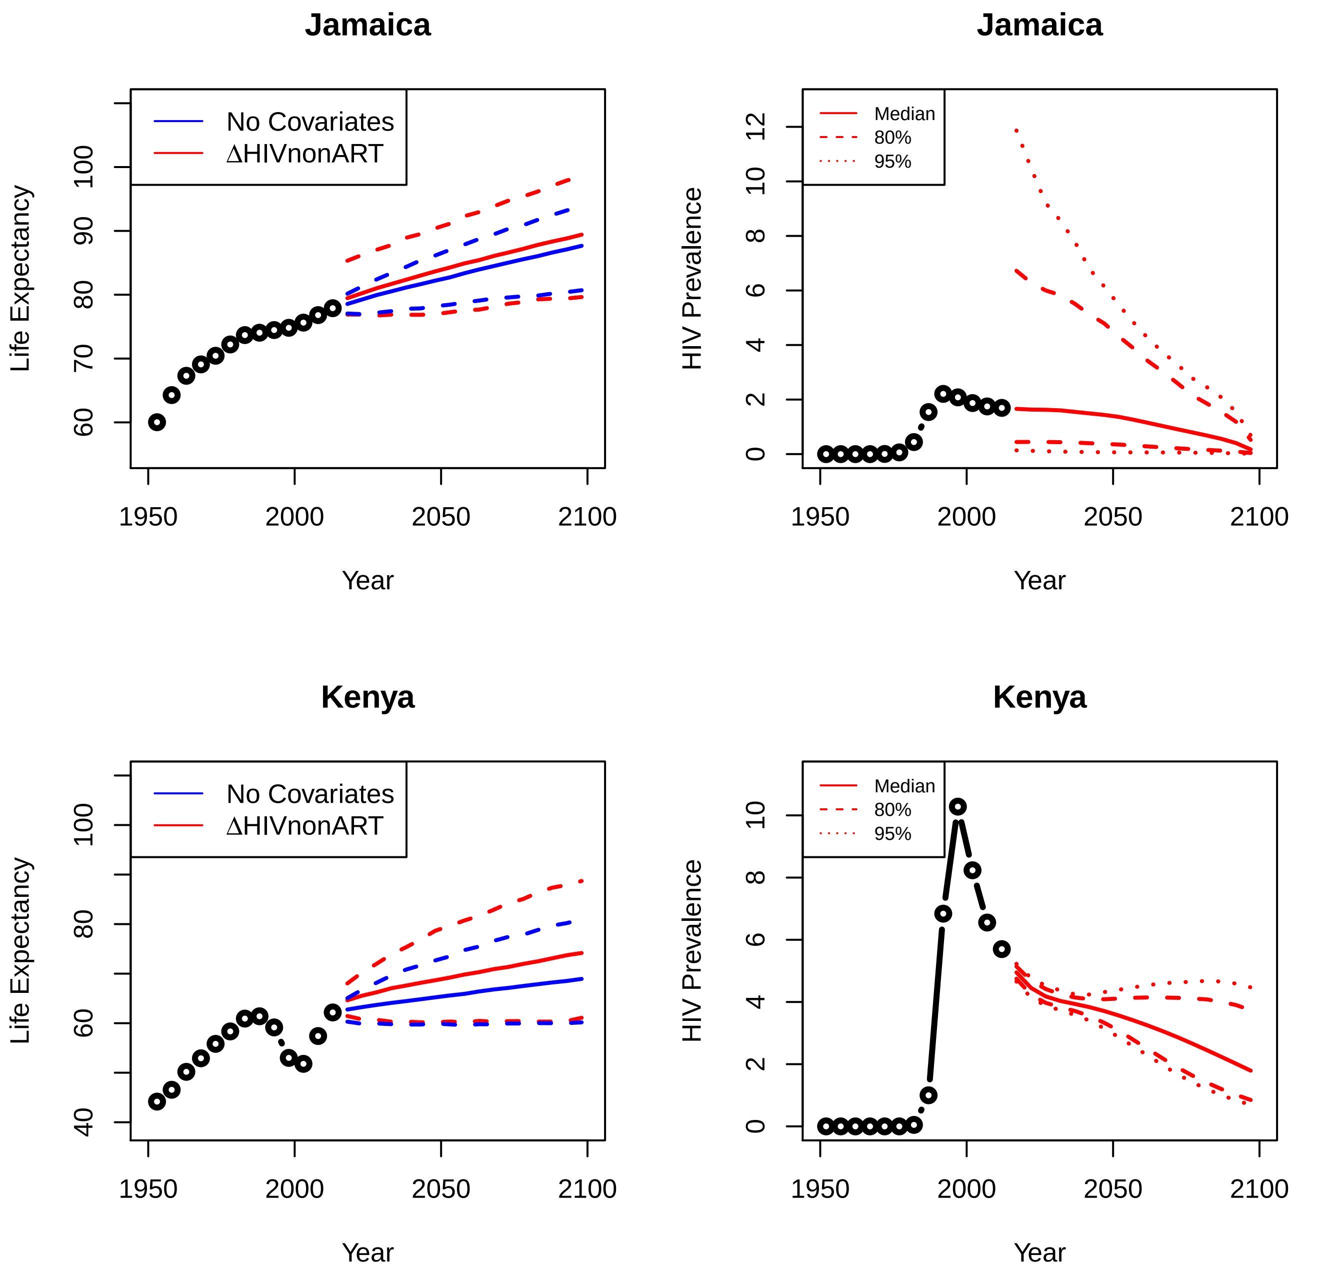

Jamaica
Life Expectancy
Year
No Covariates
ΔHIVnonART
Jamaica
HIV Prevalence
Median
80%
95%
Kenya
Life Expectancy
Kenya
HIV Prevalence
1950
2000
2050
2100

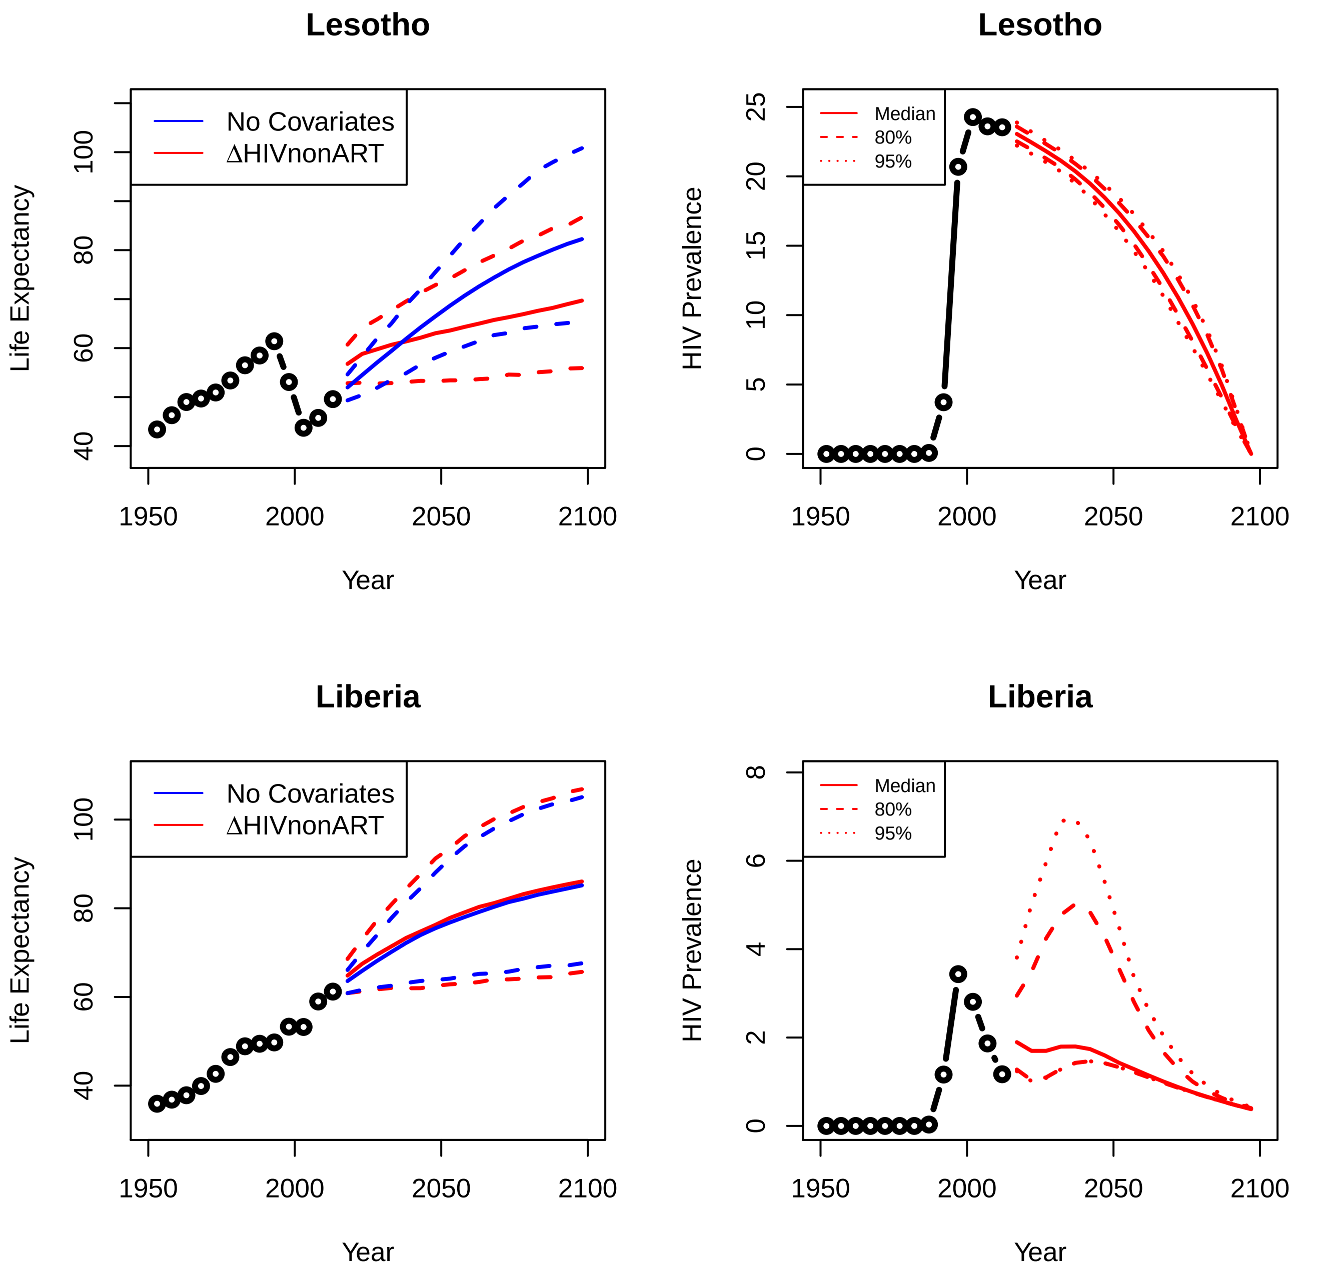

Lesotho
Life Expectancy
Year
No Covariates
ΔHIVnonART
40
60
80
100
1950
2000
2050
2100
Lesotho
HIV Prevalence
Year
Median
80%
95%
0
5
10
15
20
25
1950
2000
2050
2100
Liberia
Life Expectancy
Year
No Covariates
ΔHIVnonART
40
60
80
100
1950
2000
2050
2100
Liberia
HIV Prevalence
Year
Median
80%
95%
0
2
4
6
8
1950
2000
2050
2100

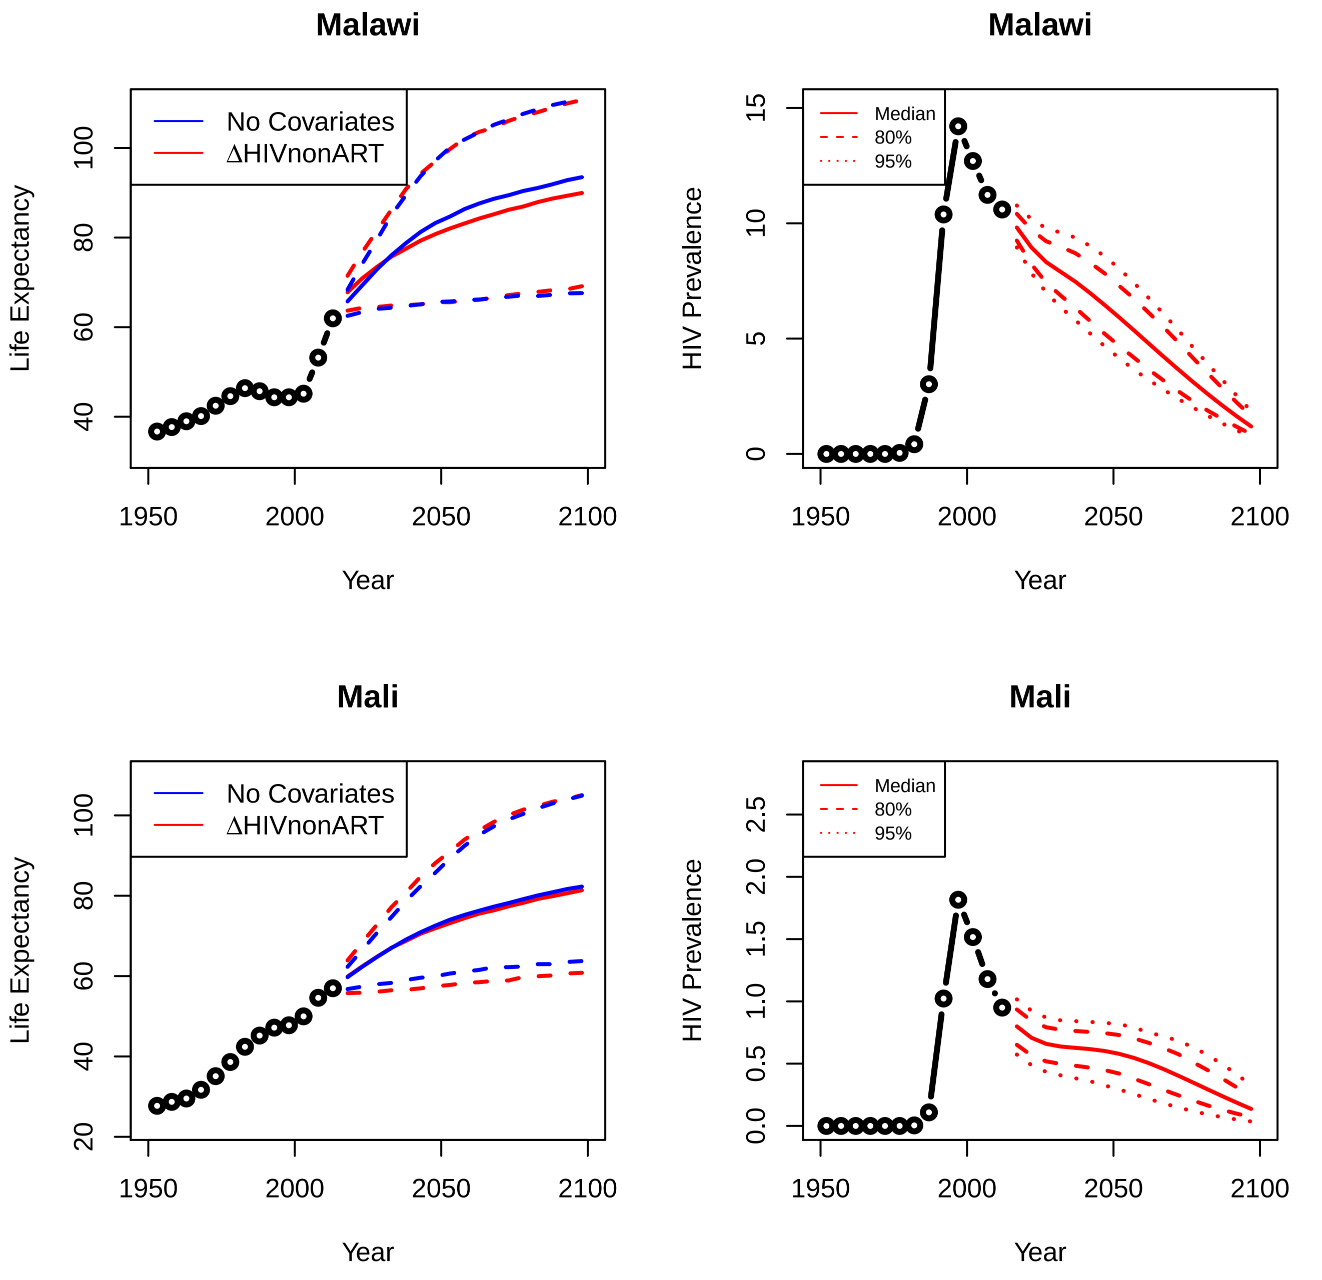
Malawi
No Covariates
ΔHIVnonART
Life Expectancy
Year
Malawi
Median
80%
95%
HIV Prevalence
Year
Mali
No Covariates
ΔHIVnonART
Life Expectancy
Year
Mali
Median
80%
95%
HIV Prevalence
Year

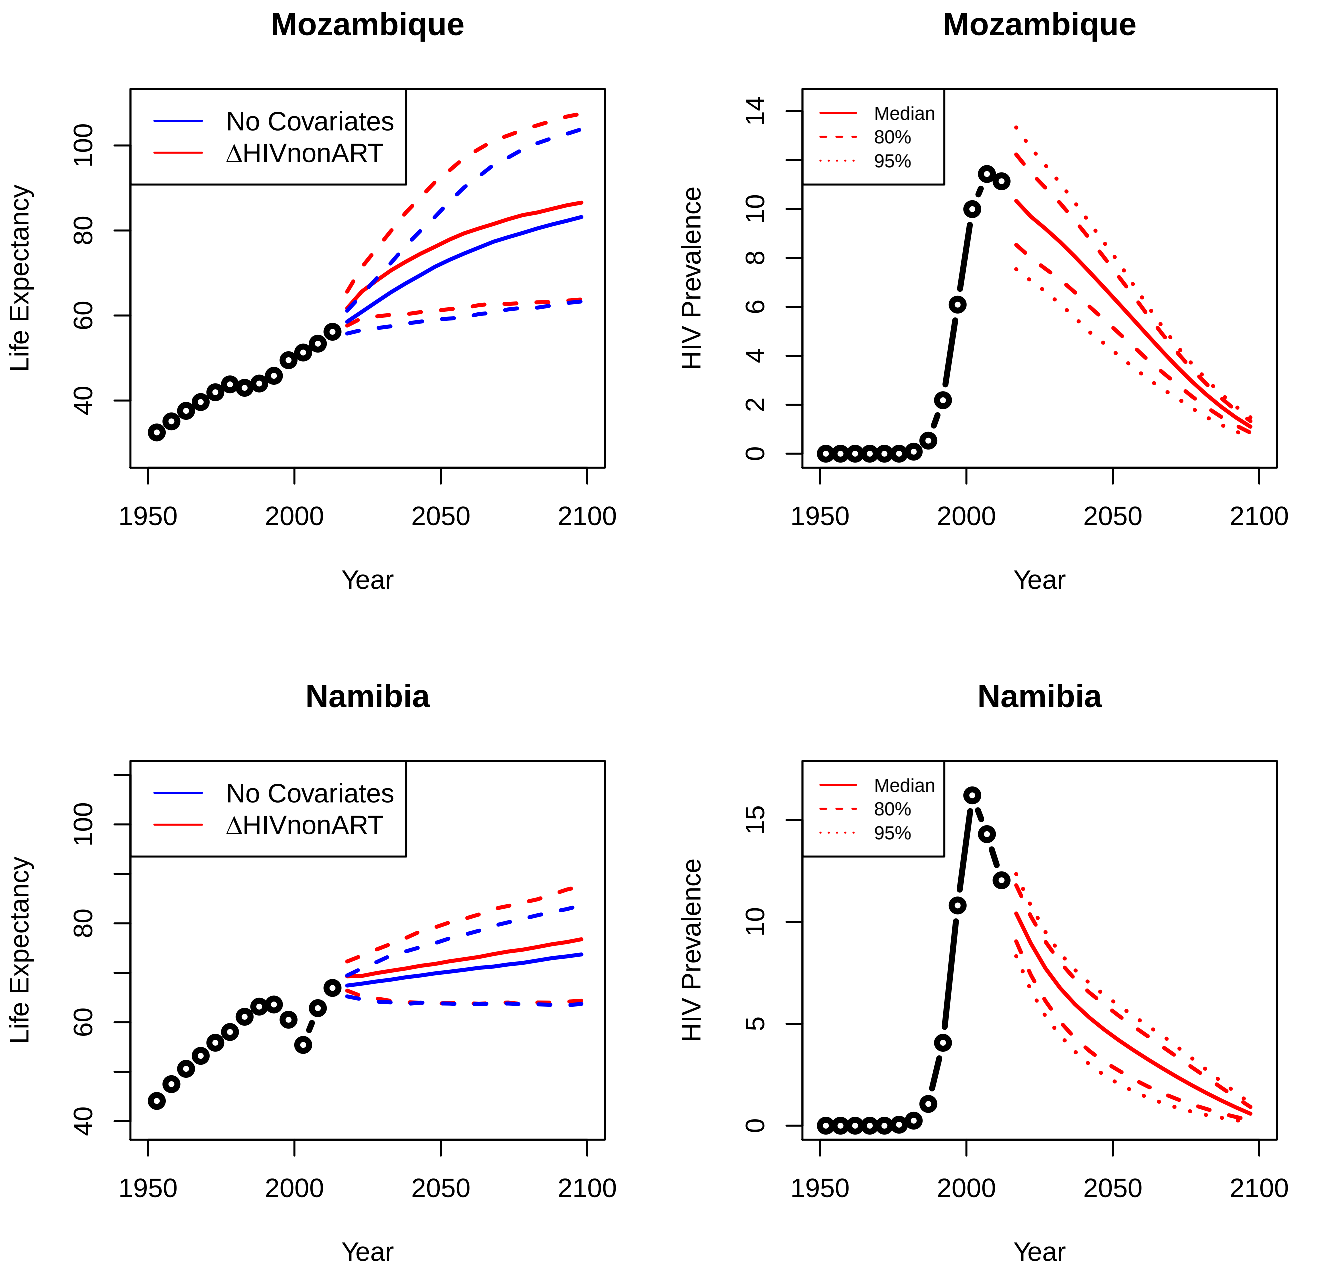
Mozambique
Life Expectancy
Year
No Covariates
ΔHIVnonART
40
60
80
100
1950
2000
2050
2100
Mozambique
HIV Prevalence
Year
Median
80%
95%
0
2
4
6
8
10
14
1950
2000
2050
2100
Namibia
Life Expectancy
Year
No Covariates
ΔHIVnonART
40
60
80
100
1950
2000
2050
2100
Namibia
HIV Prevalence
Year
Median
80%
95%
0
5
10
15
1950
2000
2050
2100

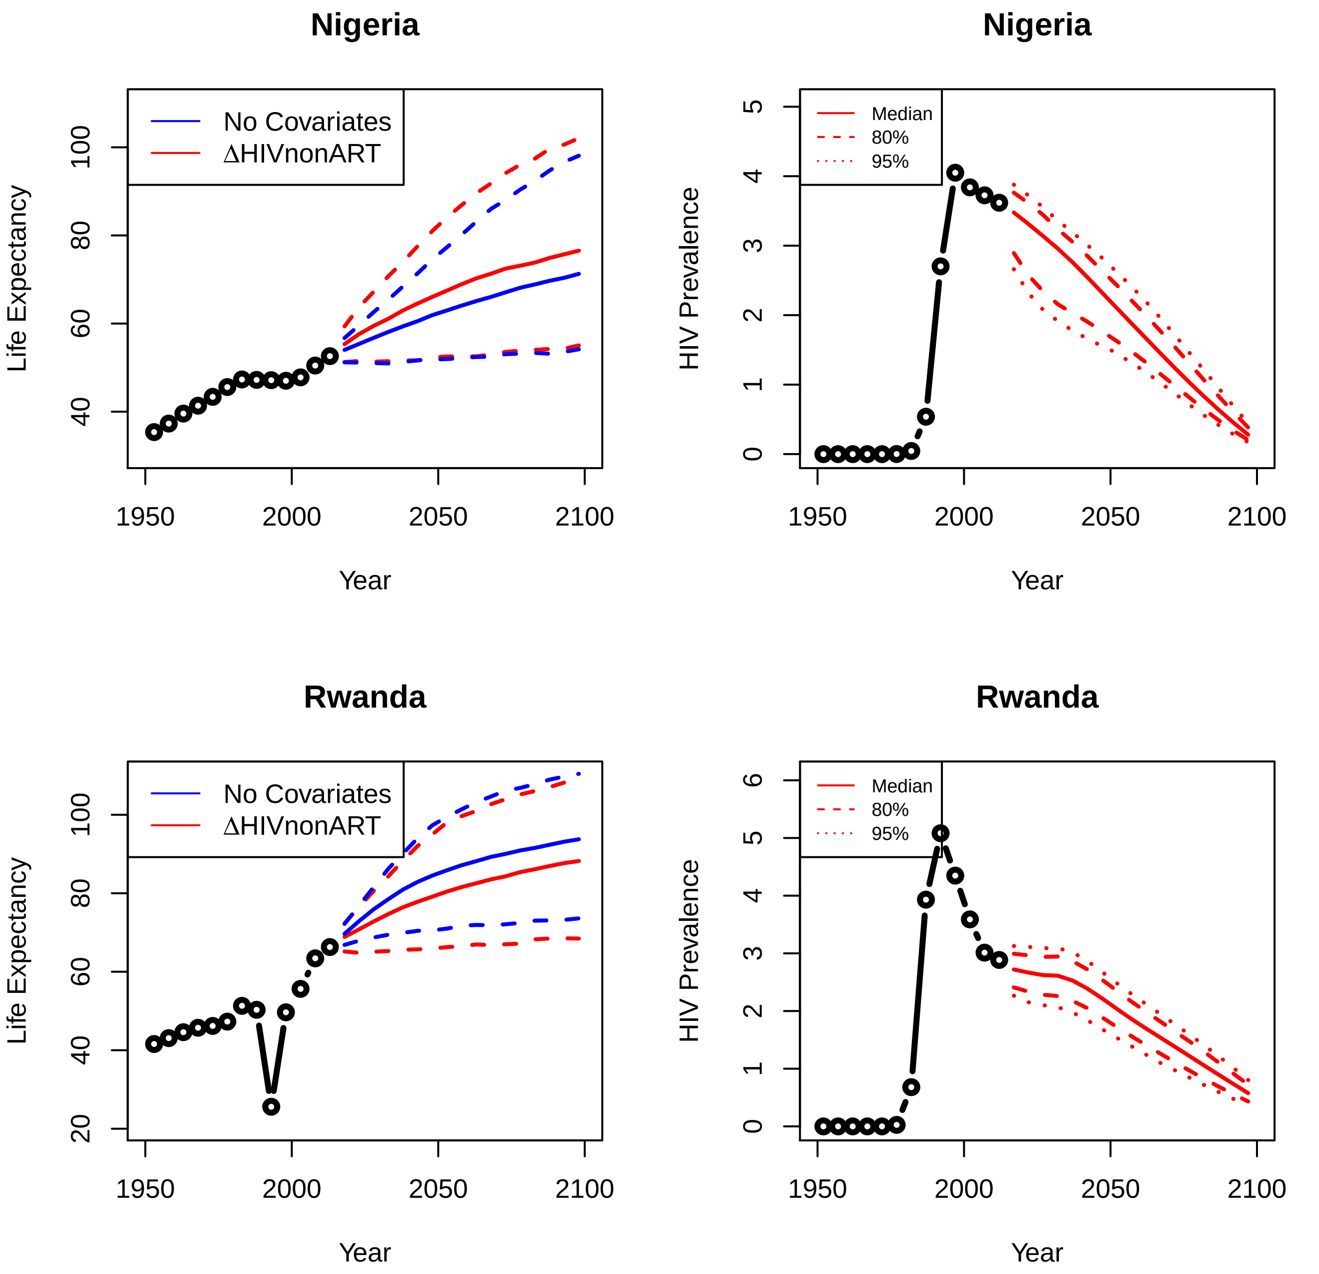
Nigeria
Life Expectancy
Year
No Covariates
ΔHIVnonART
40
60
80
100
1950
2000
2050
2100
Nigeria
HIV Prevalence
Year
Median
80%
95%
0
1
2
3
4
5
1950
2000
2050
2100
Rwanda
Life Expectancy
Year
No Covariates
ΔHIVnonART
20
40
60
80
100
1950
2000
2050
2100
Rwanda
HIV Prevalence
Year
Median
80%
95%
0
1
2
3
4
5
6
1950
2000
2050
2100

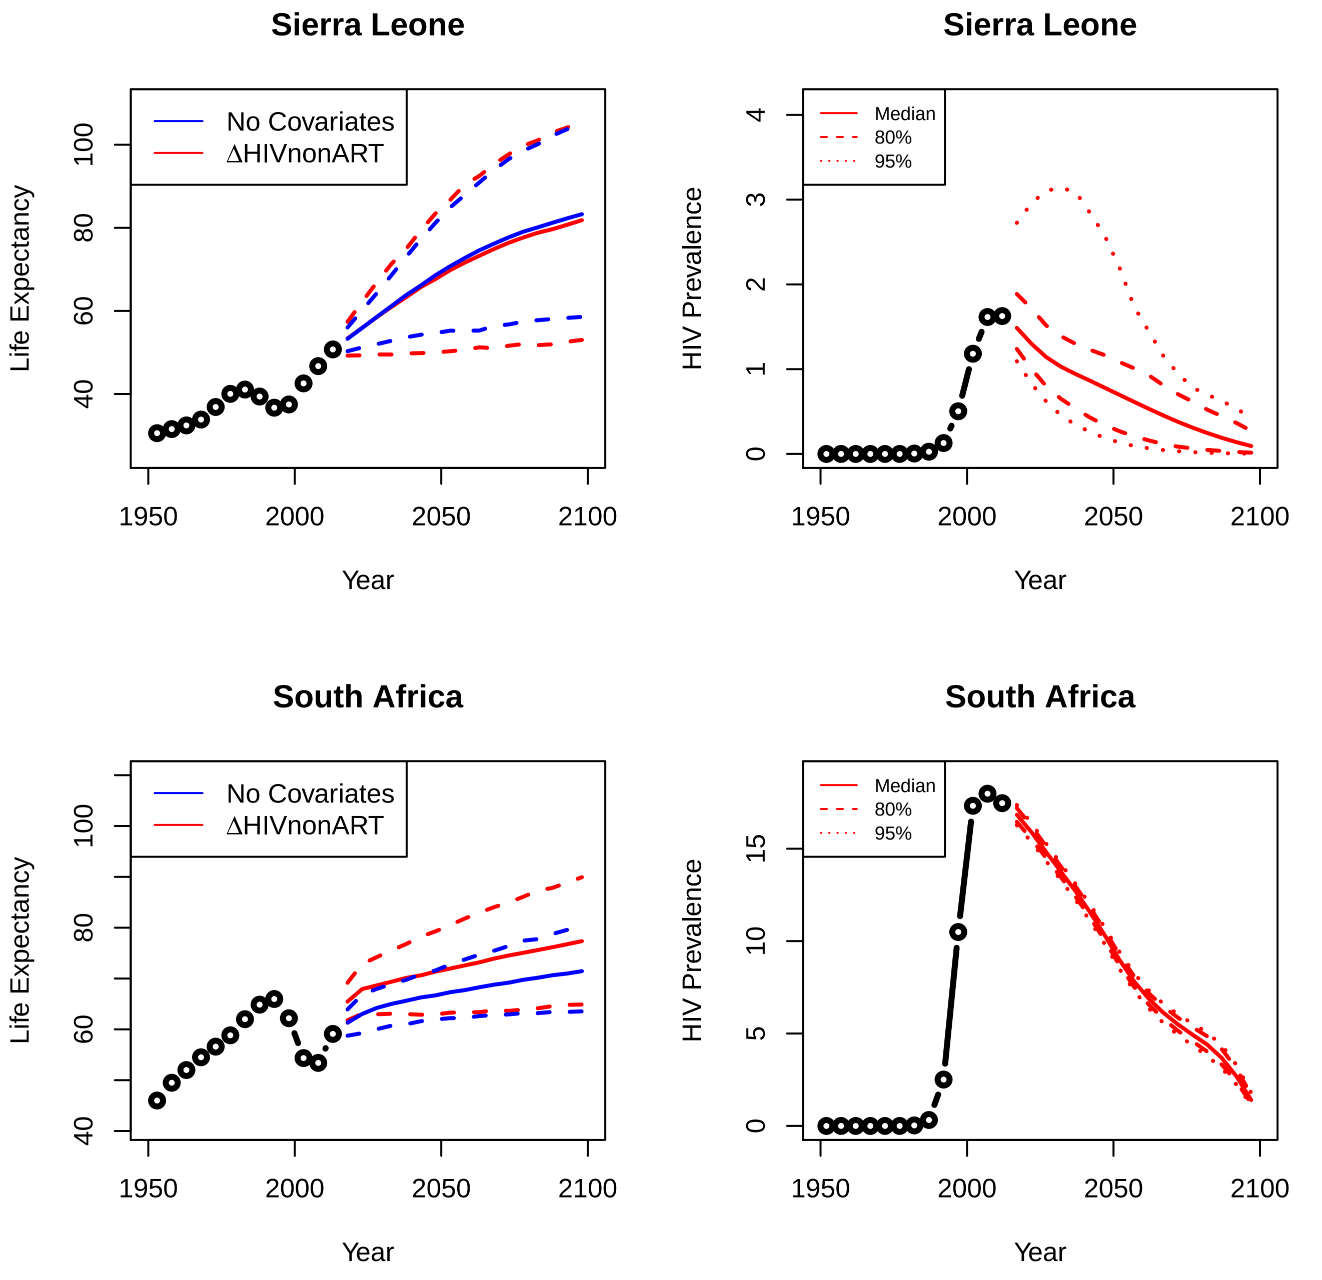

Sierra Leone
Life Expectancy
No Covariates
ΔHIVnonART
Year
Sierra Leone
HIV Prevalence
Median
80%
95%
Year
South Africa
Life Expectancy
No Covariates
ΔHIVnonART
Year
South Africa
HIV Prevalence
Median
80%
95%
Year

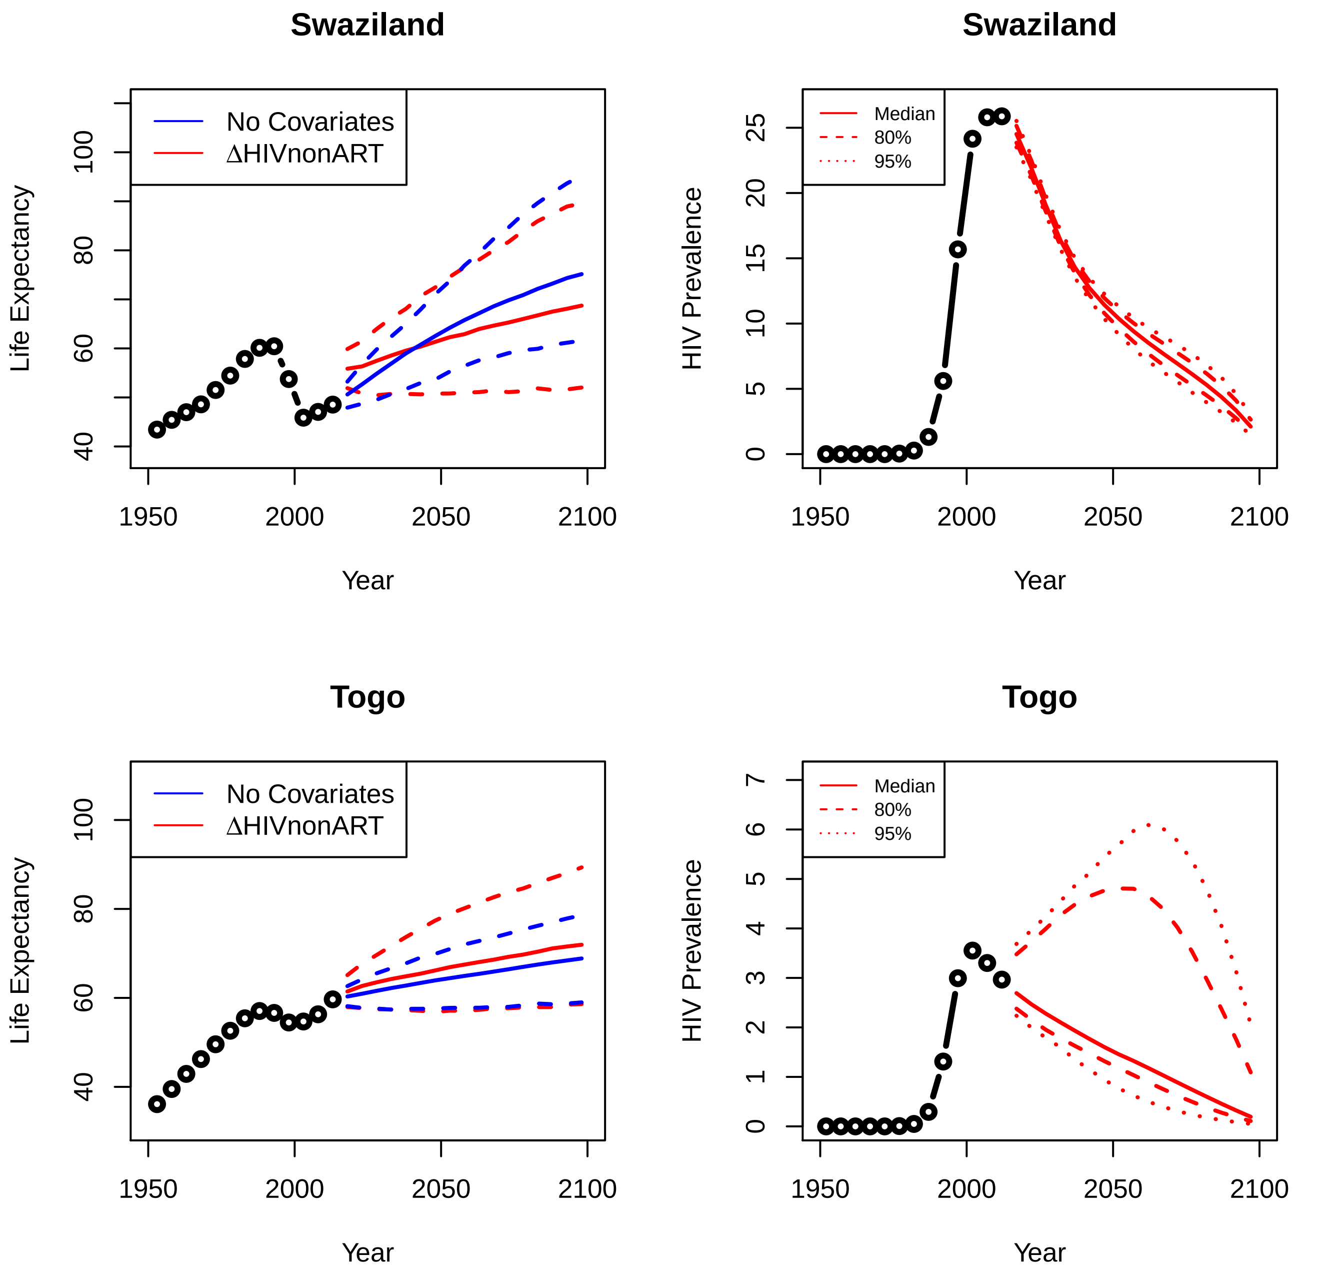

Swaziland
No Covariates
ΔHIVnonART
Life Expectancy
Year
Swaziland
Median
80%
95%
HIV Prevalence
Year
Togo
No Covariates
ΔHIVnonART
Life Expectancy
Year
Togo
Median
80%
95%
HIV Prevalence
Year

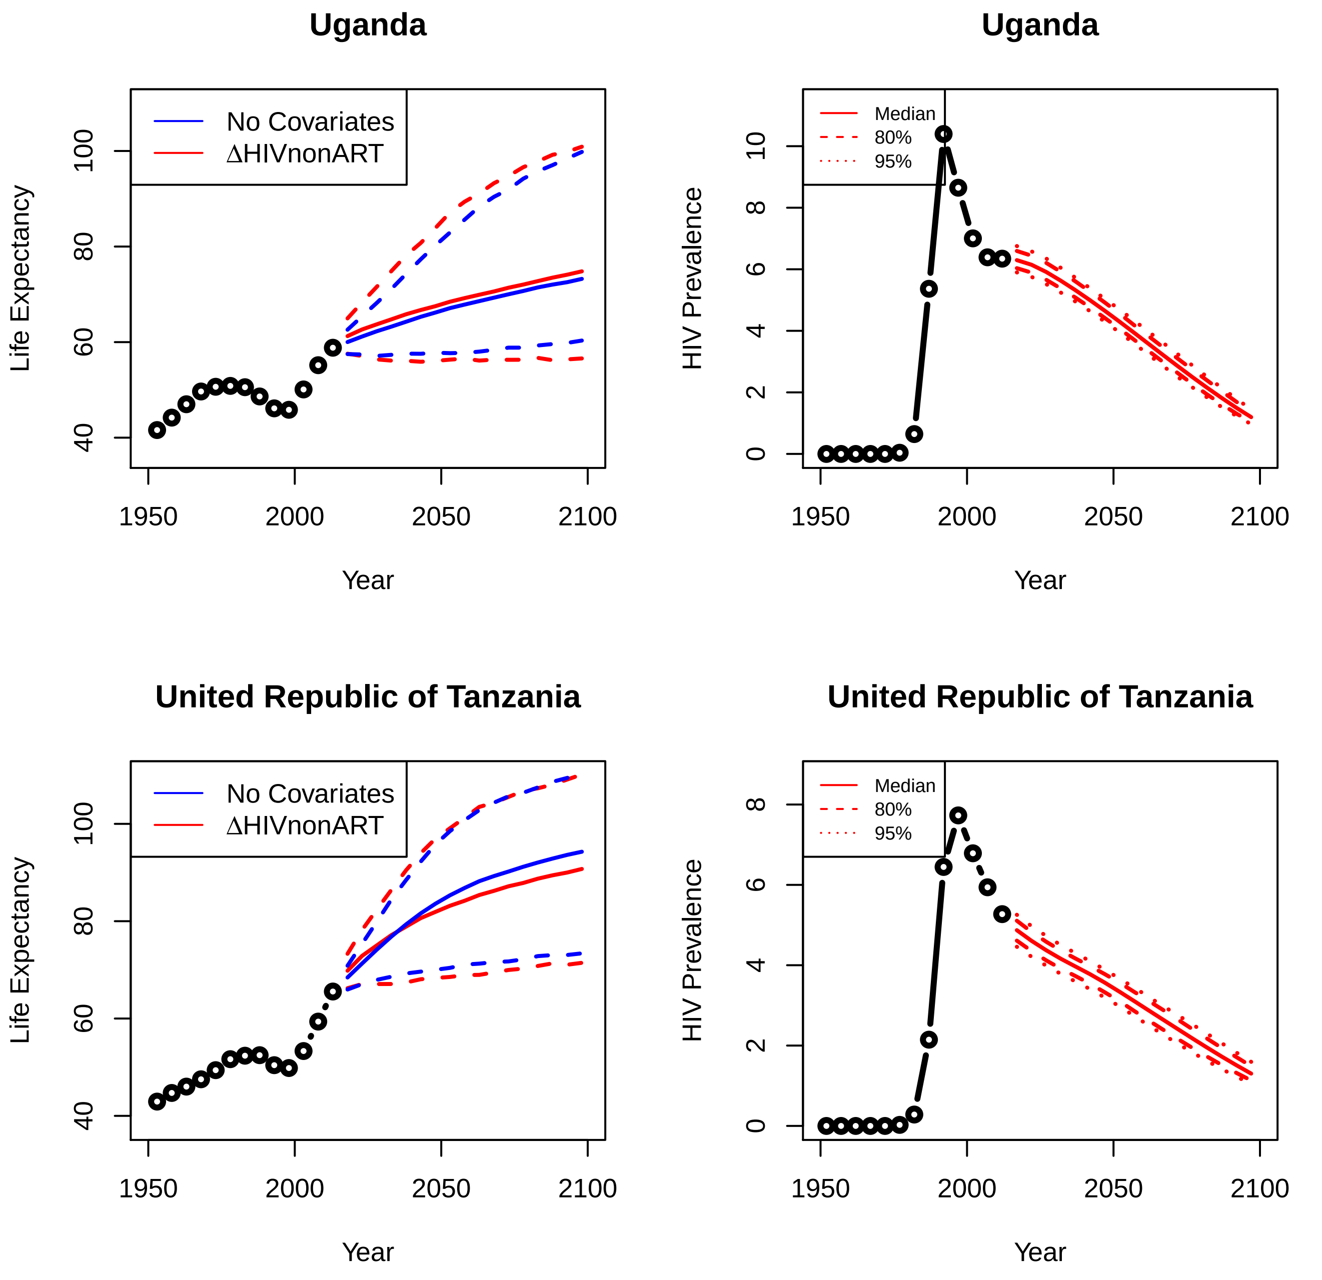
Uganda
No Covariates
ΔHIVnonART
Life Expectancy
Year
40
60
80
100
1950
2000
2050
2100
Uganda
Median
80%
95%
HIV Prevalence
Year
0
2
4
6
8
10
1950
2000
2050
2100
United Republic of Tanzania
No Covariates
ΔHIVnonART
Life Expectancy
Year
40
60
80
100
1950
2000
2050
2100
United Republic of Tanzania
Median
80%
95%
HIV Prevalence
Year
0
2
4
6
8
1950
2000
2050
2100

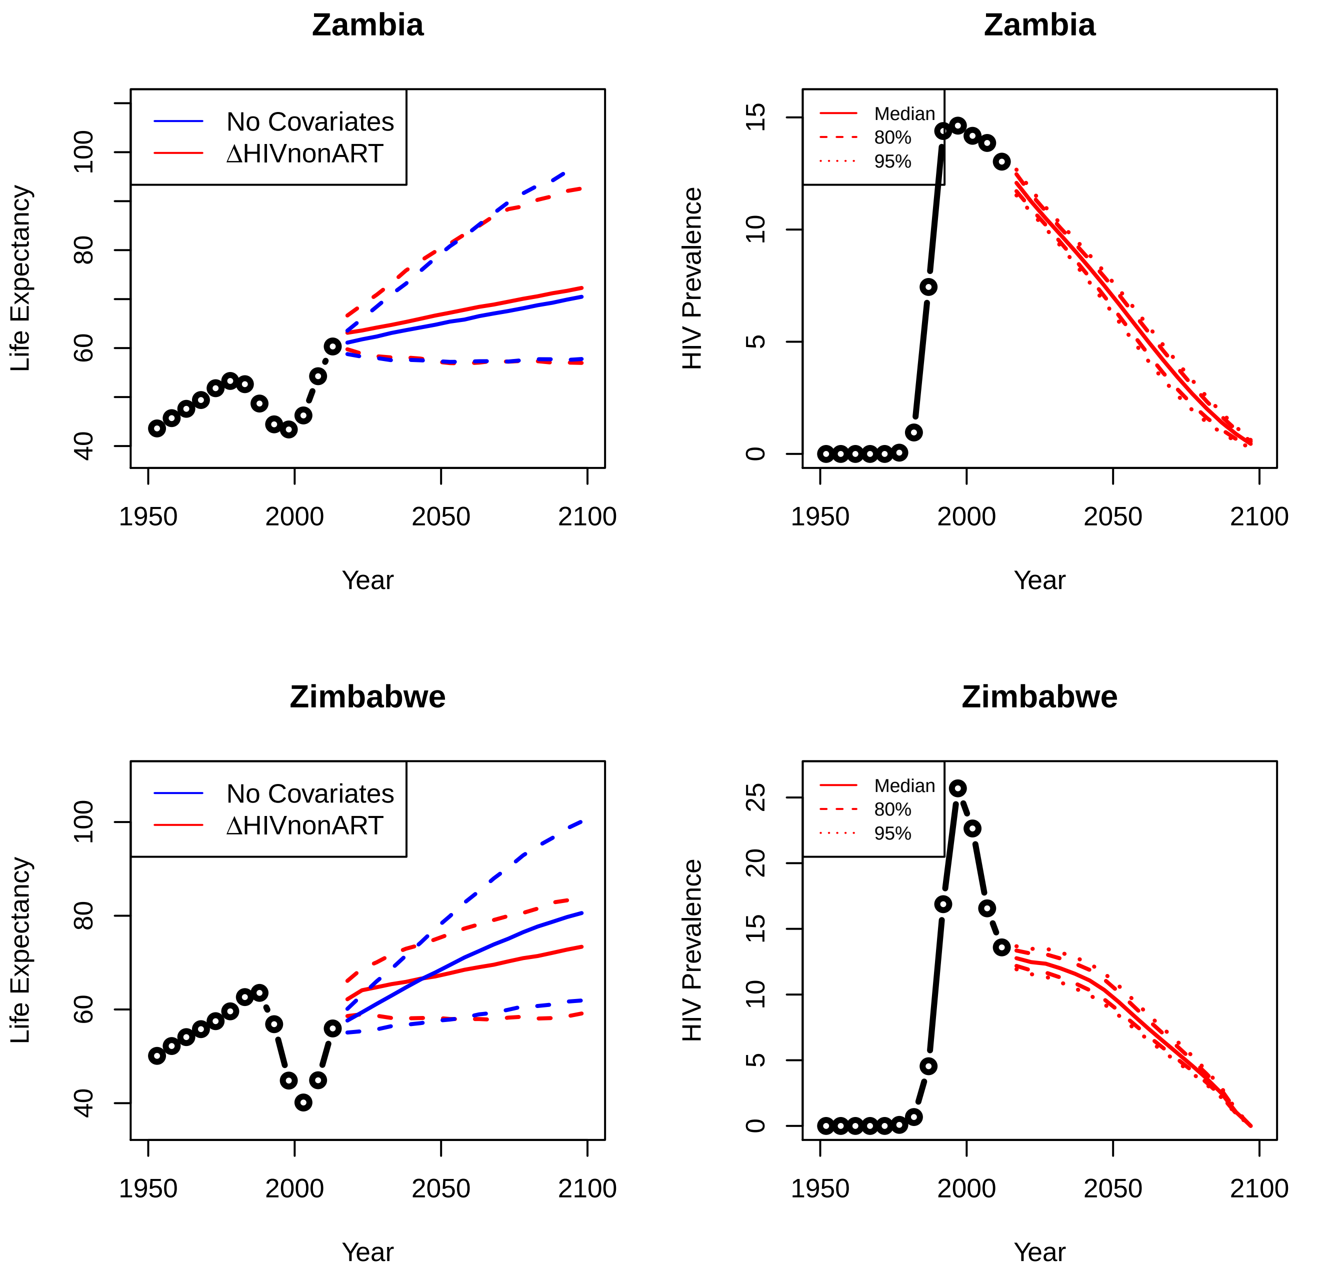
Zambia
Life Expectancy
No Covariates
ΔHIVnonART
Year
Zambia
HIV Prevalence
Median
80%
95%
Year
Zimbabwe
Life Expectancy
No Covariates
ΔHIVnonART
Year
Zimbabwe
HIV Prevalence
Median
80%
95%
Year
