# Supplementary material for: Bayesian Projection of Life Expectancy Accounting for the HIV/AIDS Epidemic
Source: arXiv:1608.07330 source file (2016-09-27)

Angola

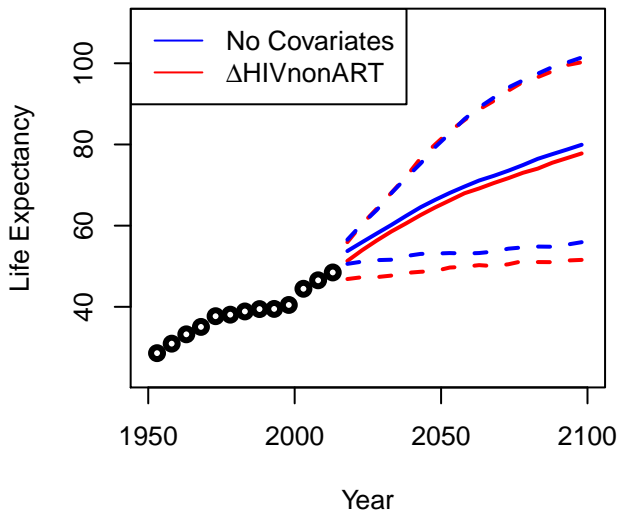

Angola

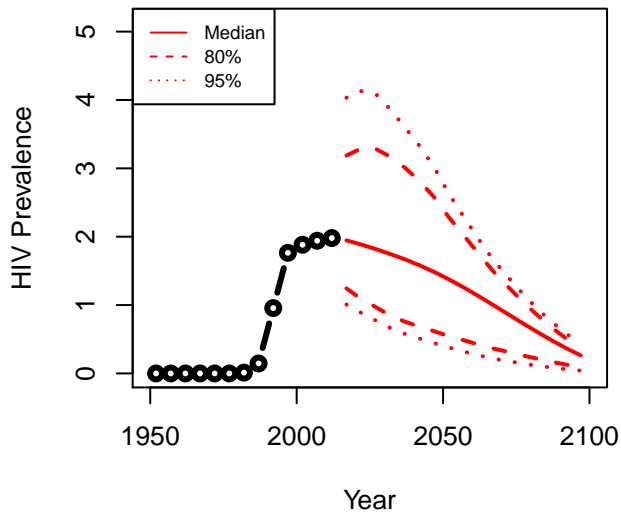

Bahamas

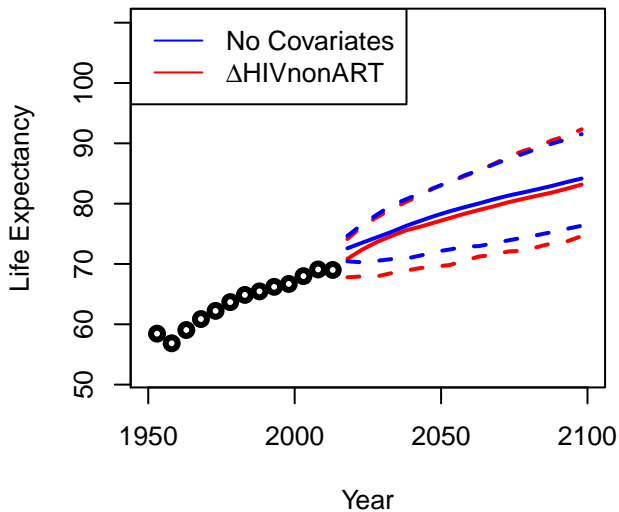

Bahamas

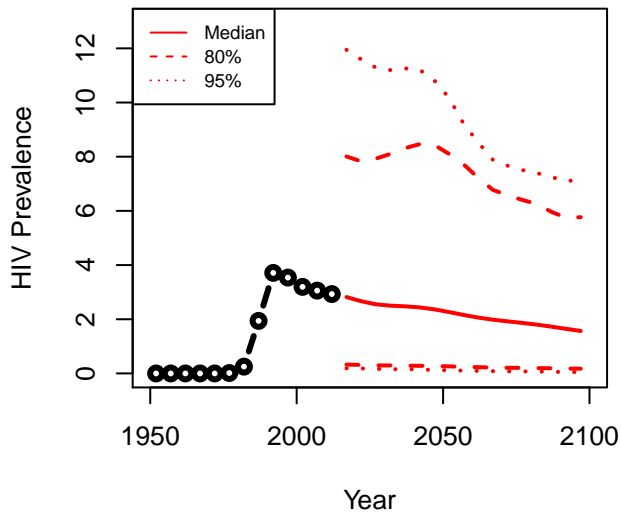

**Belize**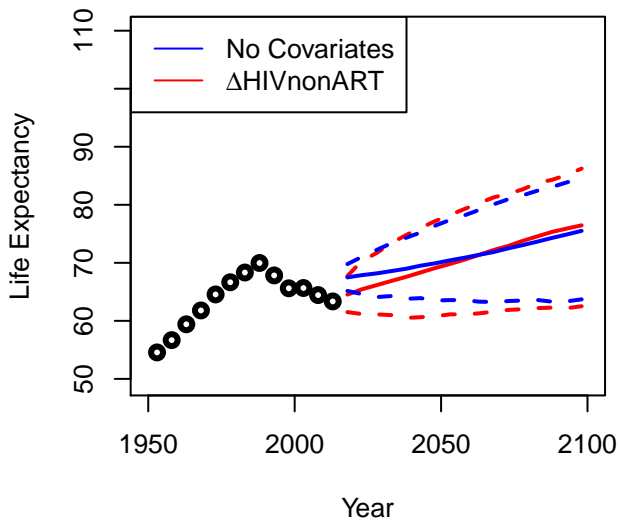**Belize**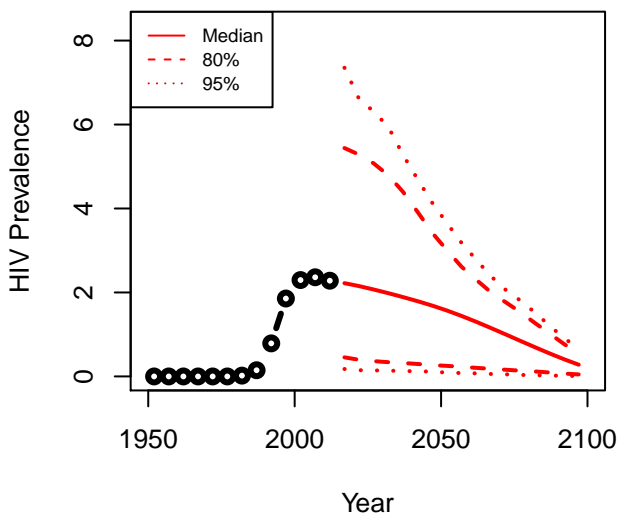**Benin**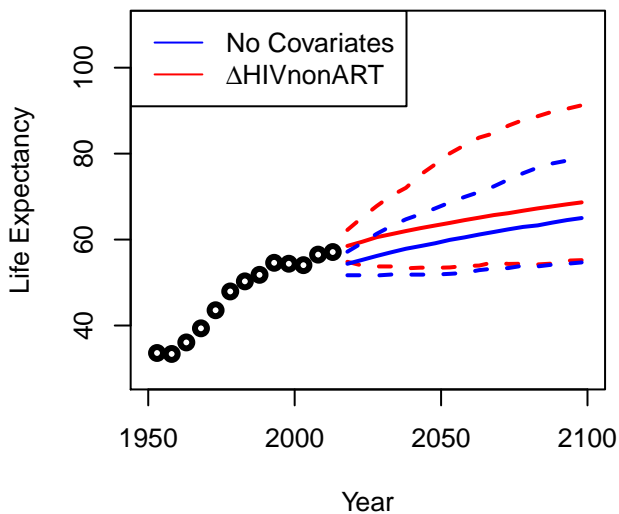**Benin**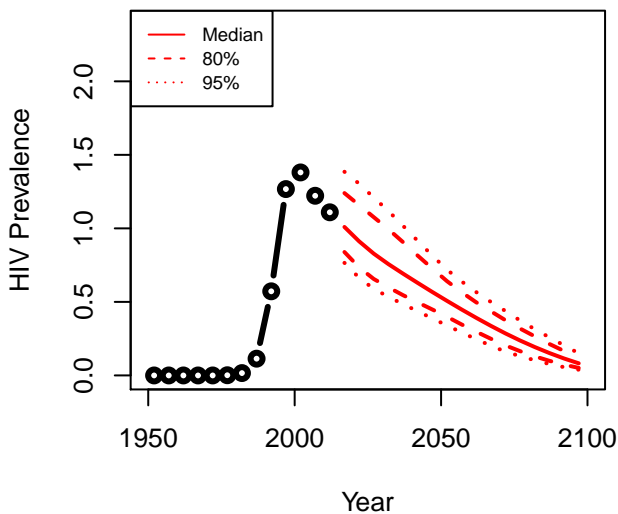

**Botswana**

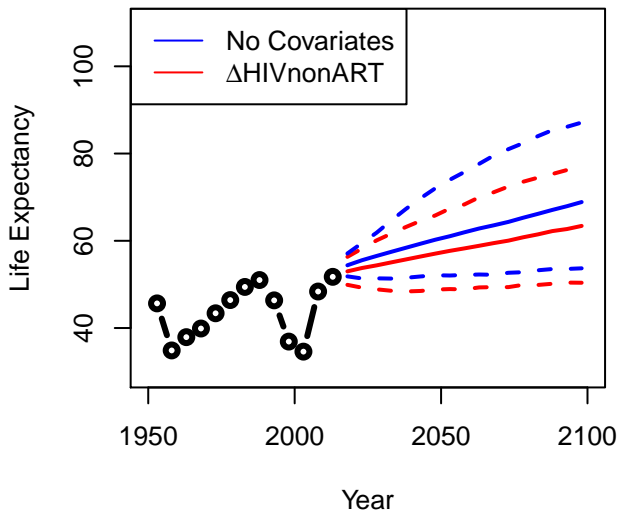

**Botswana**

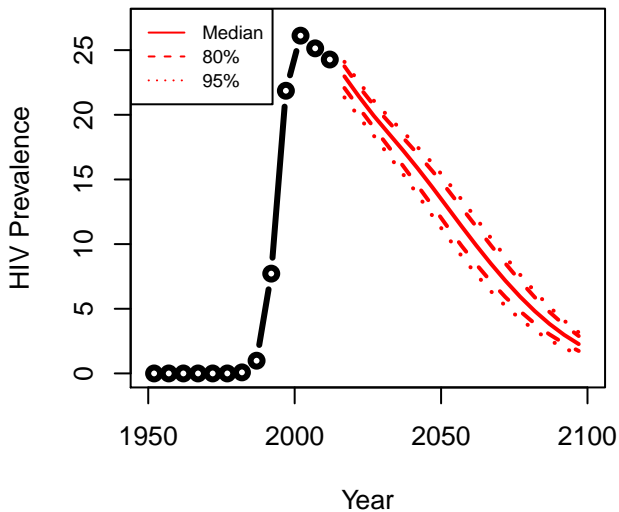

**Burkina Faso**

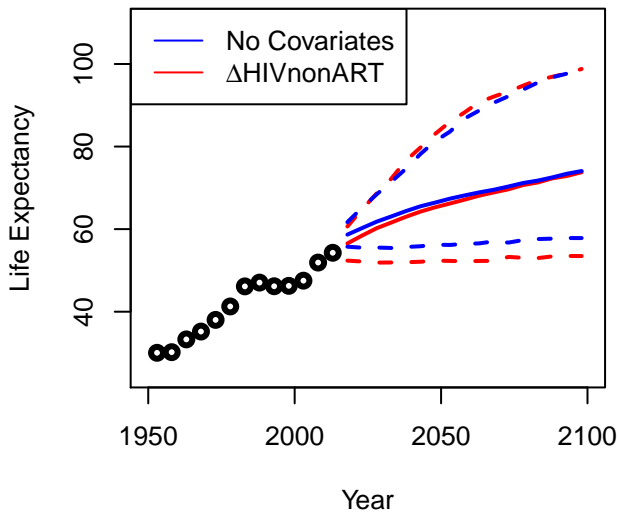

**Burkina Faso**

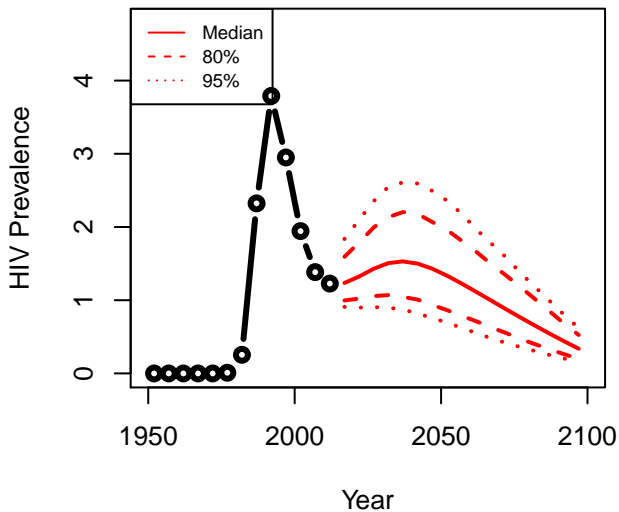

**Burundi**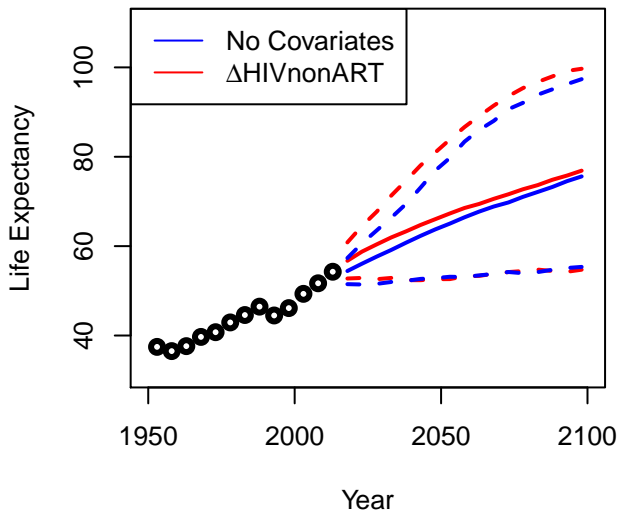**Burundi**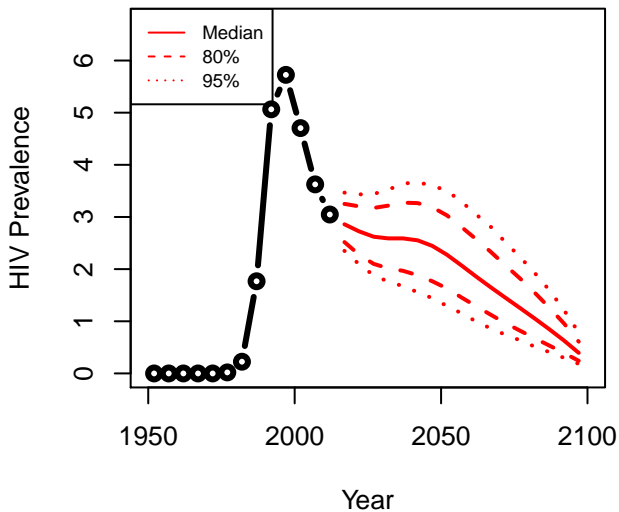**Cameroon**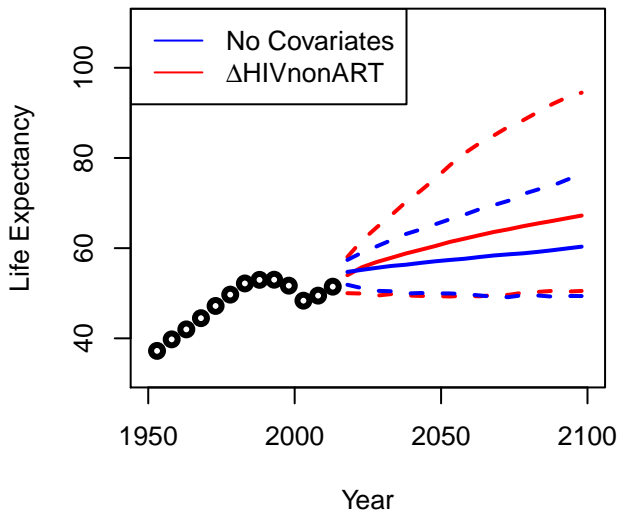**Cameroon**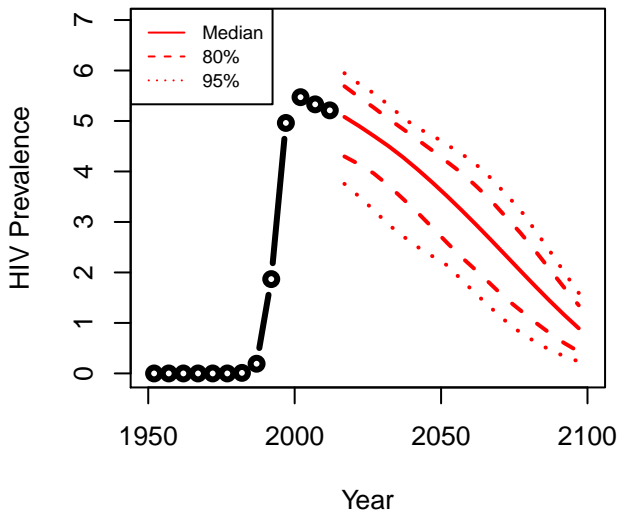

**Central African Republic**

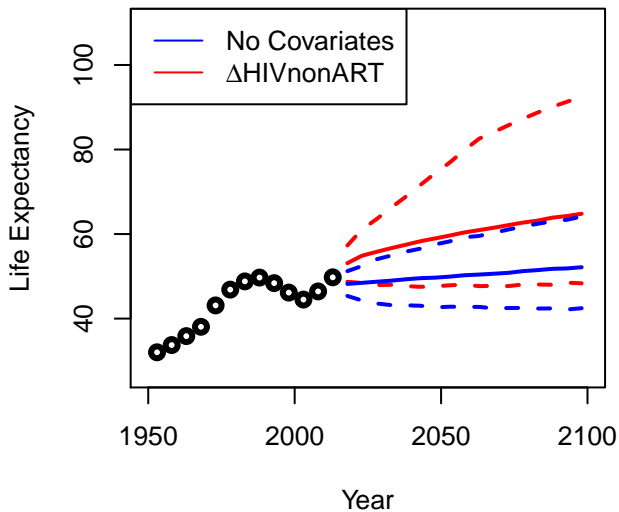

**Central African Republic**

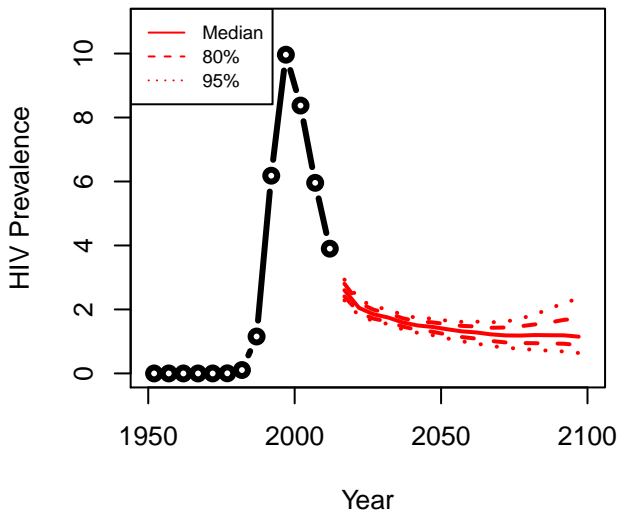

**Chad**

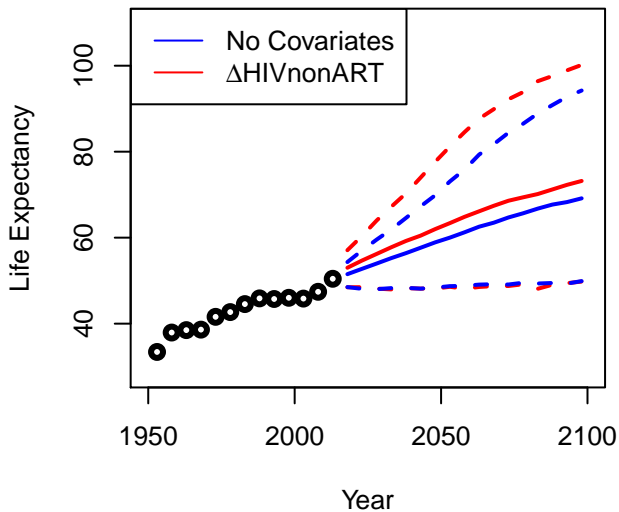

**Chad**

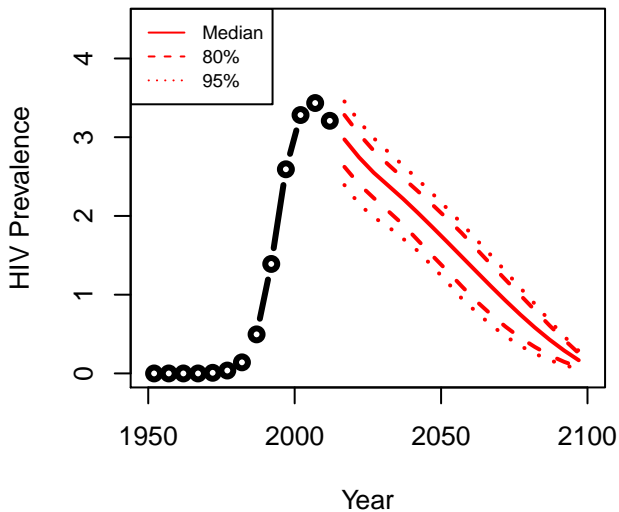

Congo

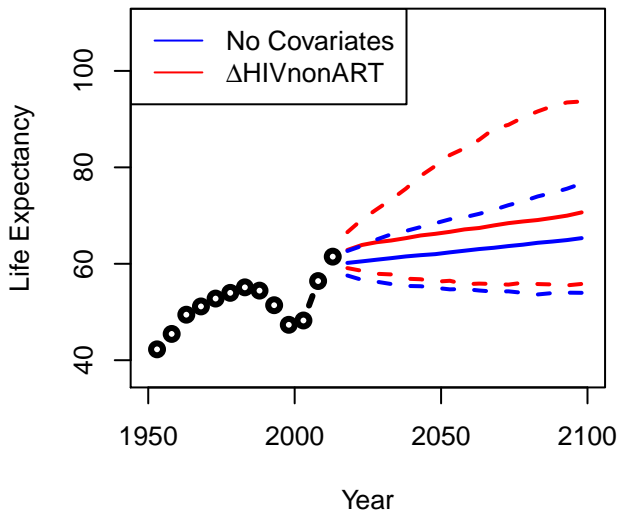

Congo

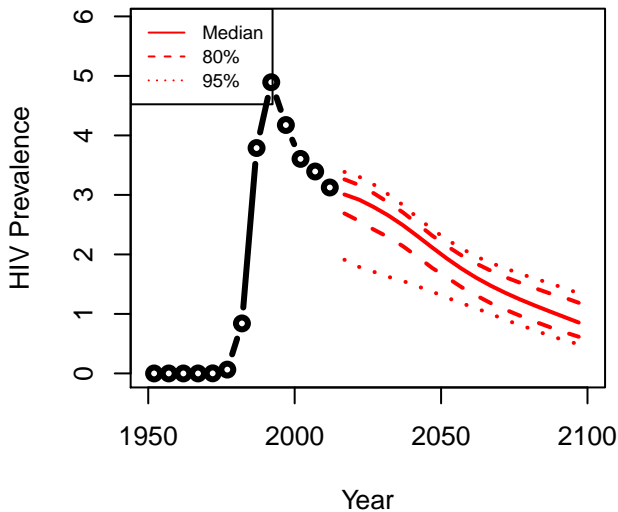

Cote d'Ivoire

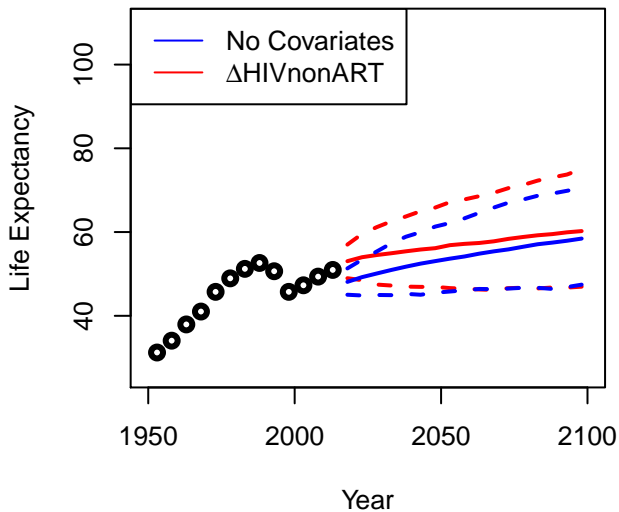

Cote d'Ivoire

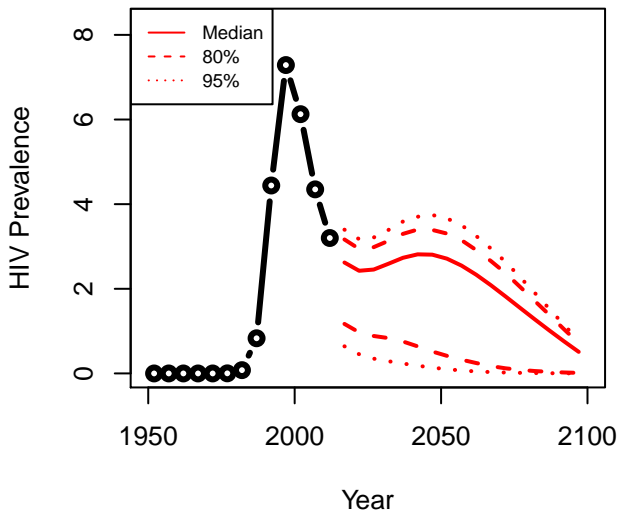

**Djibouti**

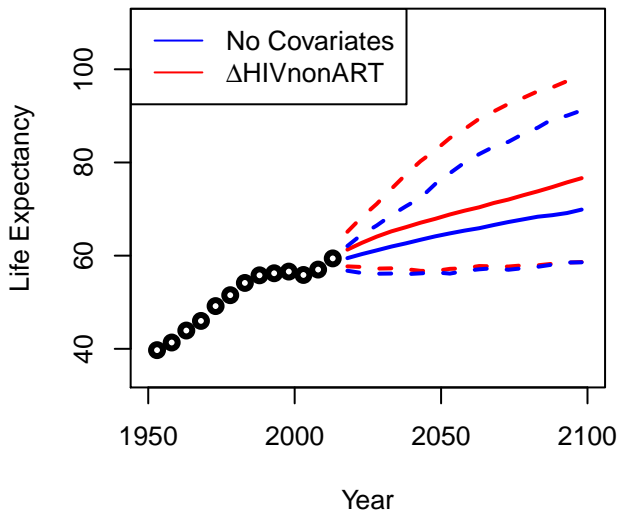

**Djibouti**

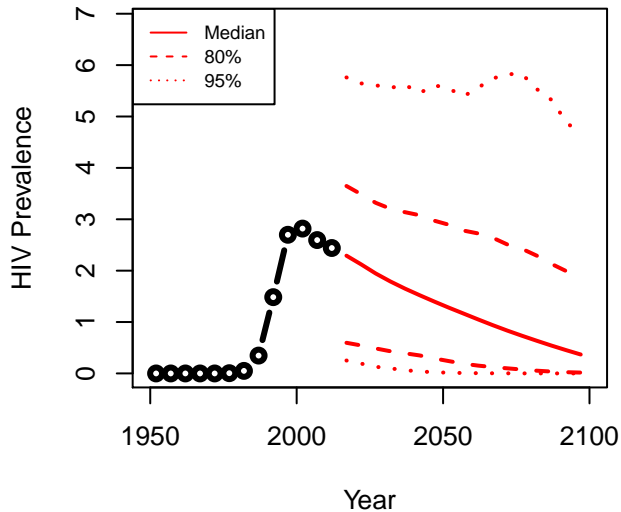

**Equatorial Guinea**

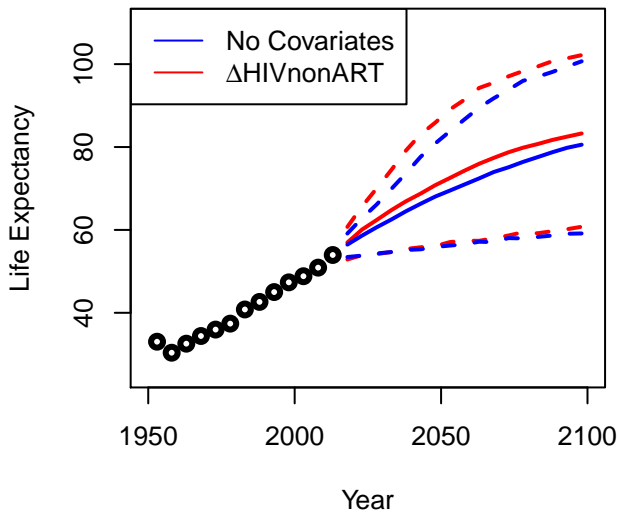

**Equatorial Guinea**

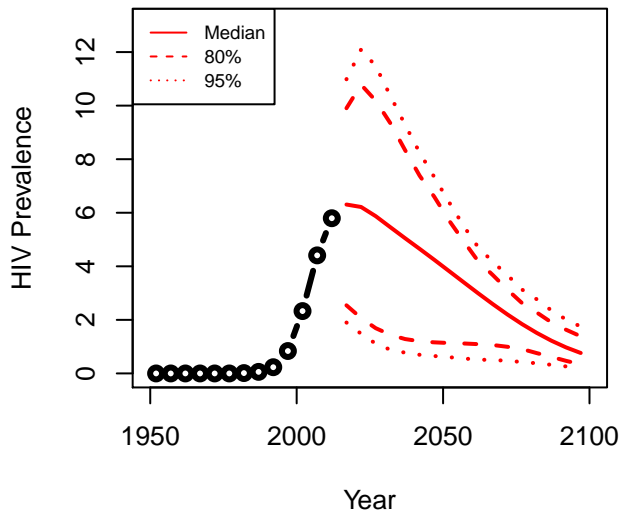

### Ethiopia

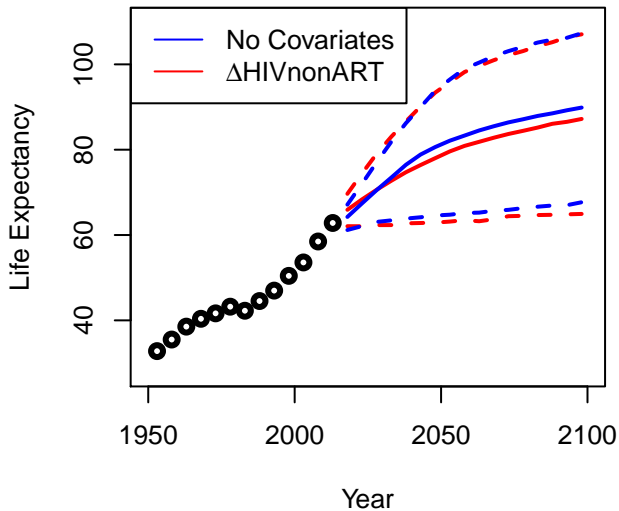

### Ethiopia

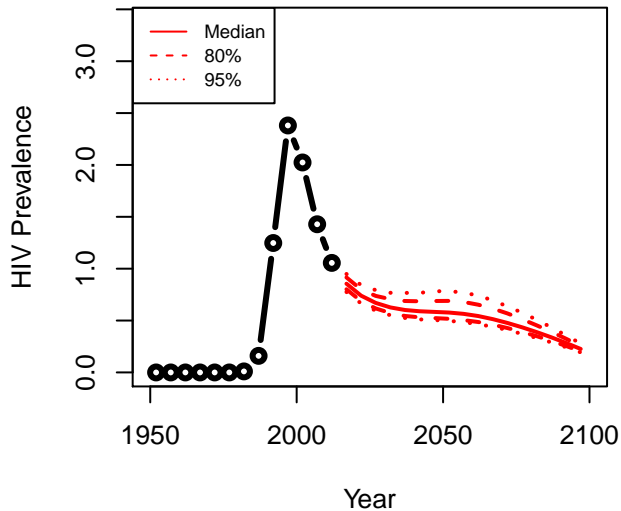

### Gabon

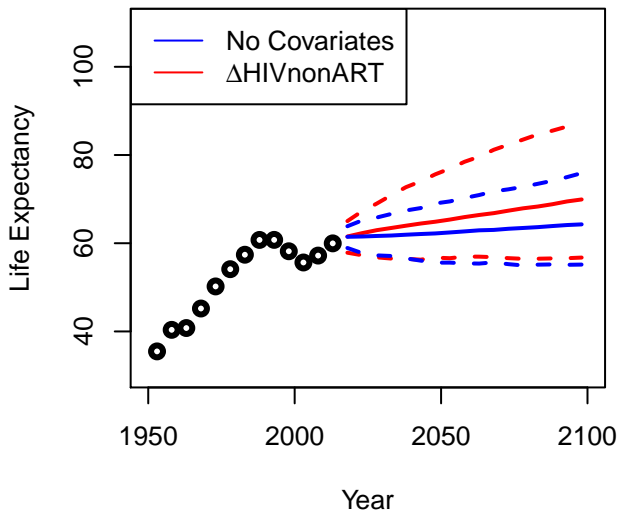

### Gabon

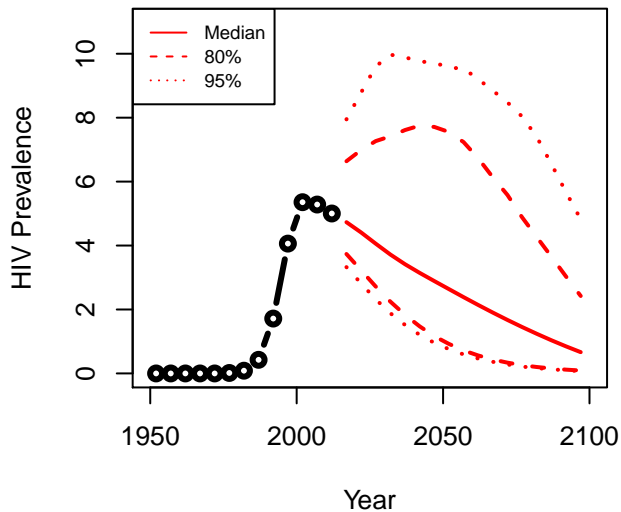



### Gambia

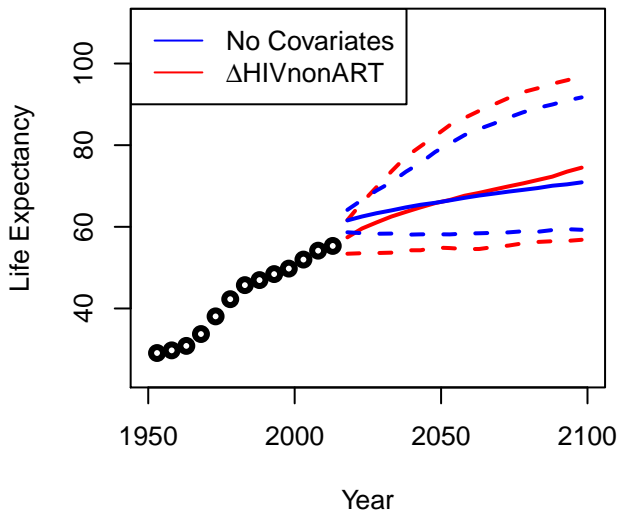

### Gambia

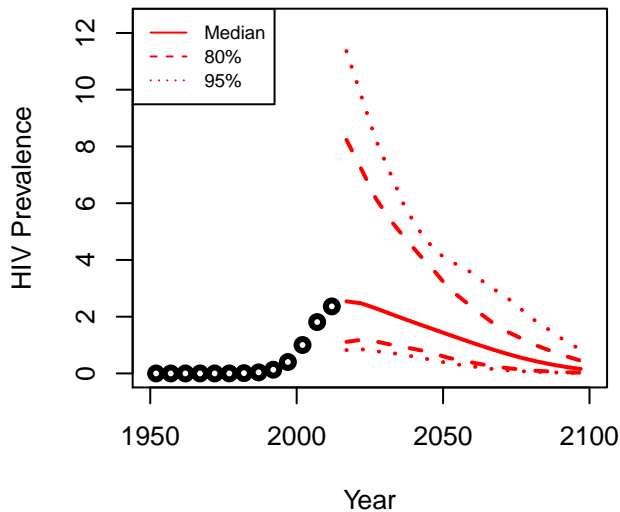

### Ghana

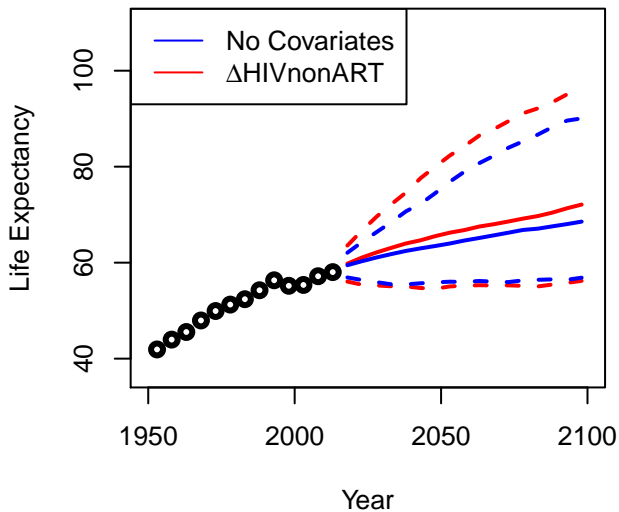

### Ghana

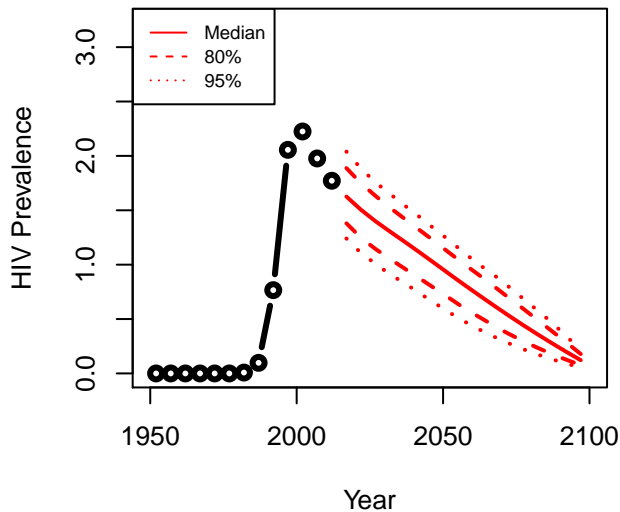

**Guinea**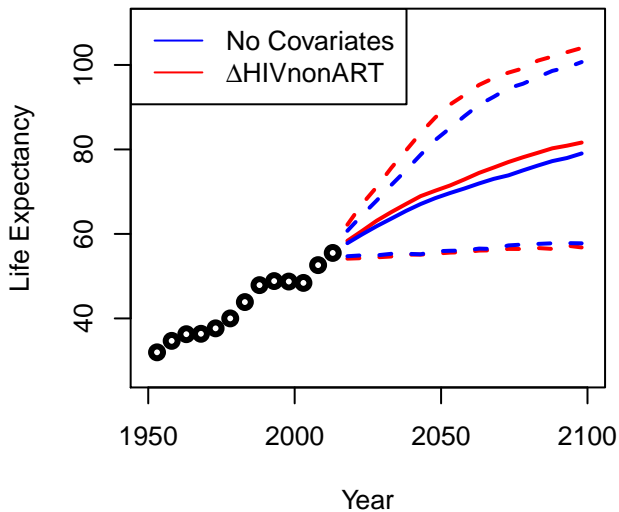**Guinea**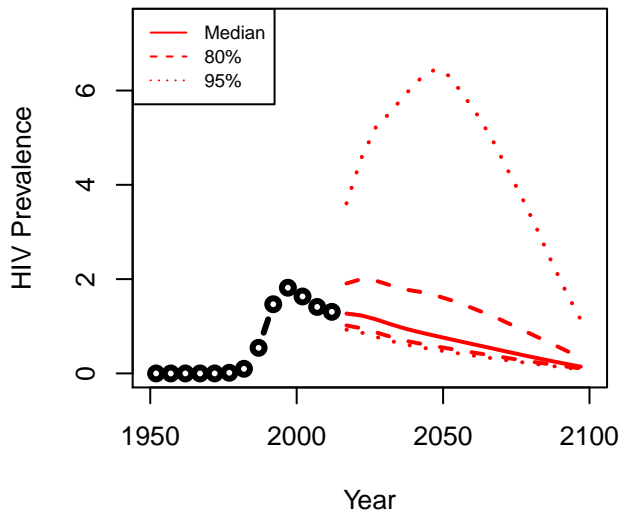**Guinea-Bissau**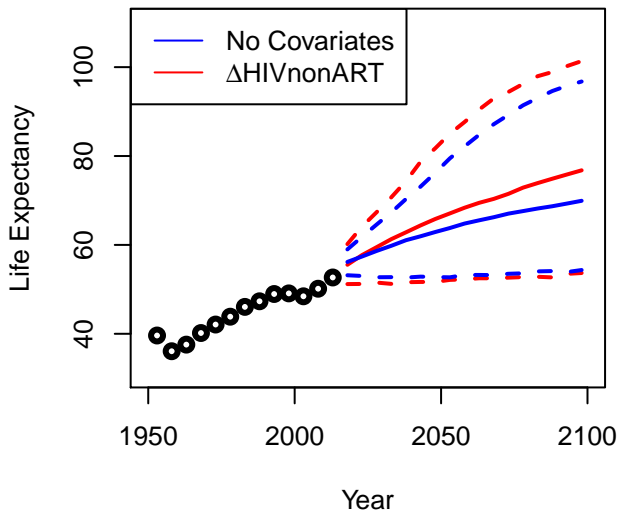**Guinea-Bissau**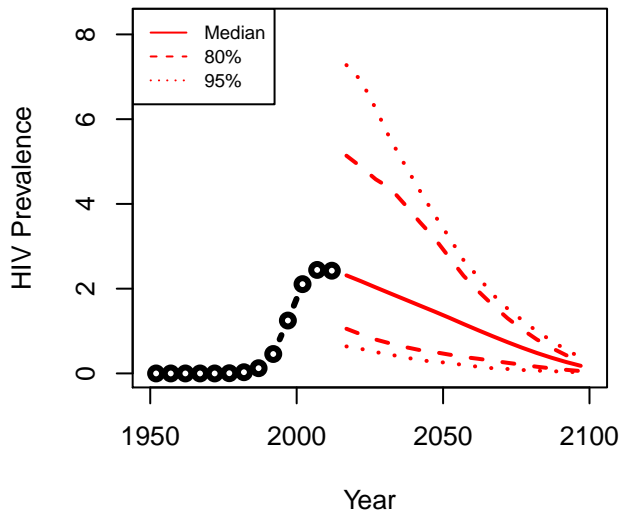

**Guyana**

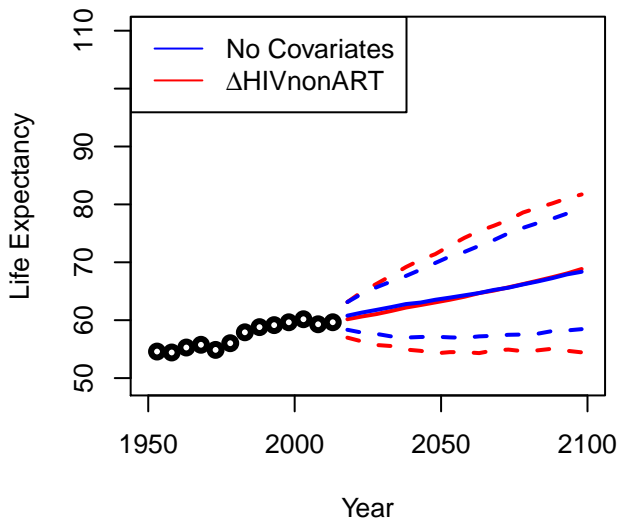

**Guyana**

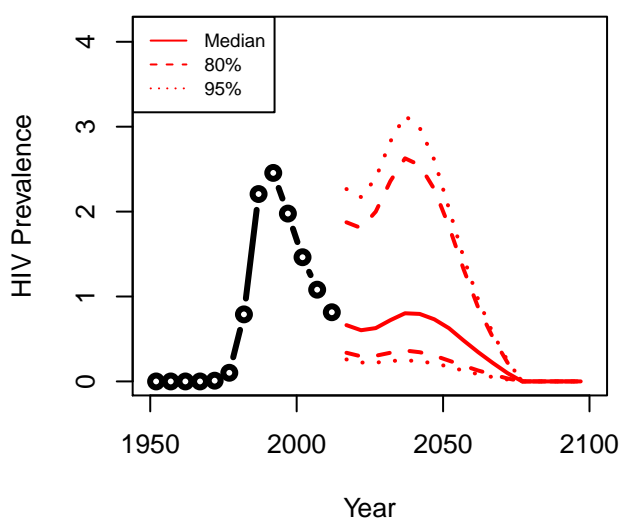

**Haiti**

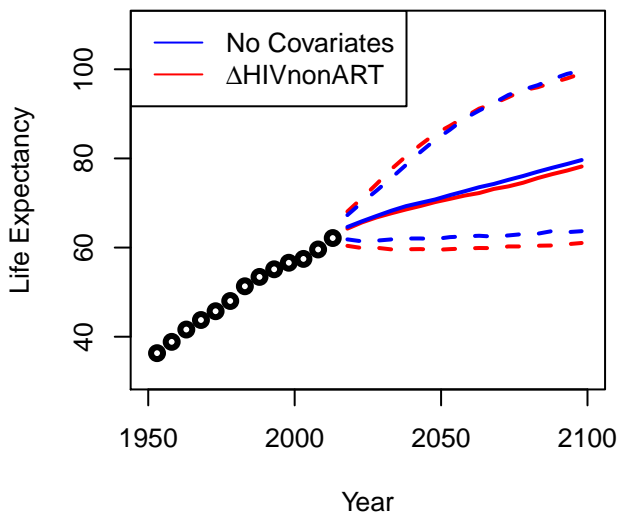

**Haiti**

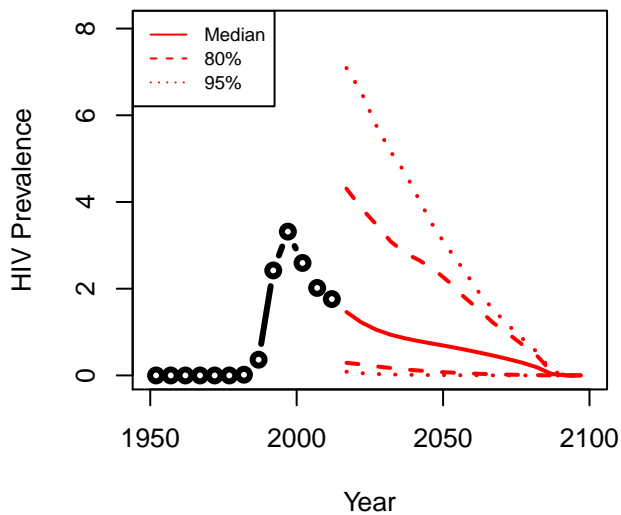

# Jamaica

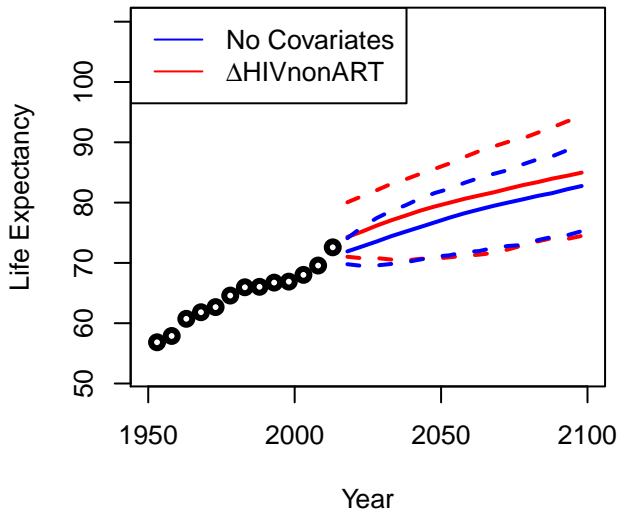

# Jamaica

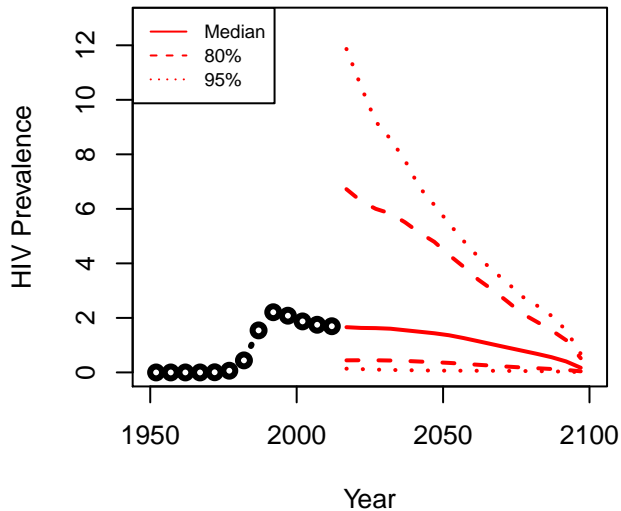

# Kenya

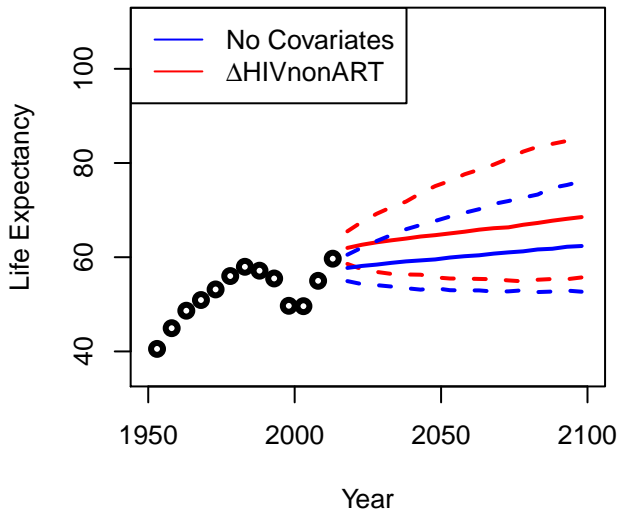

# Kenya

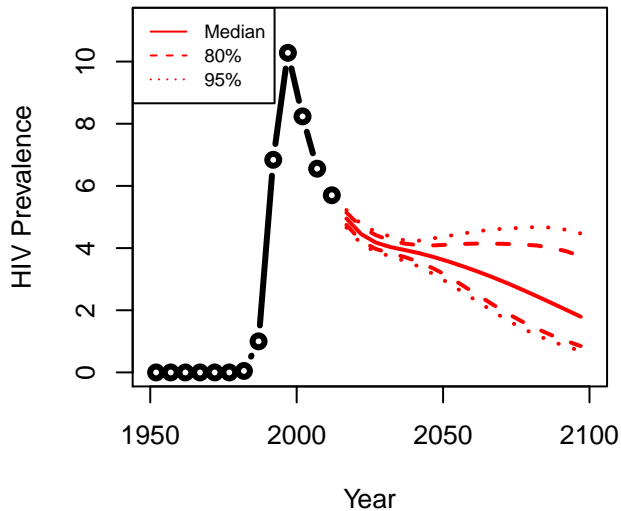

**Lesotho**

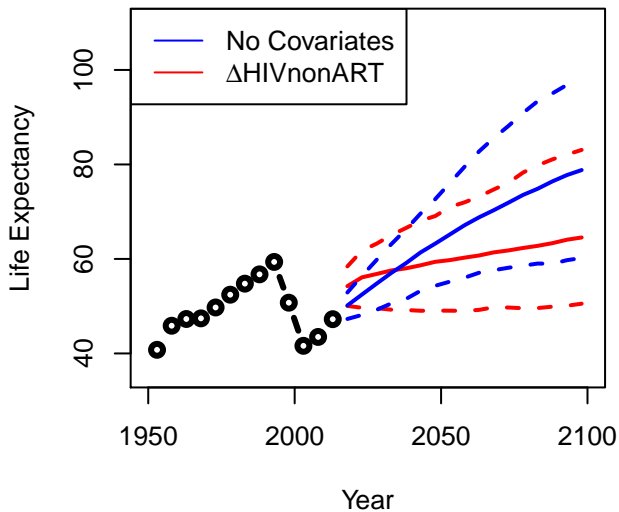

**Lesotho**

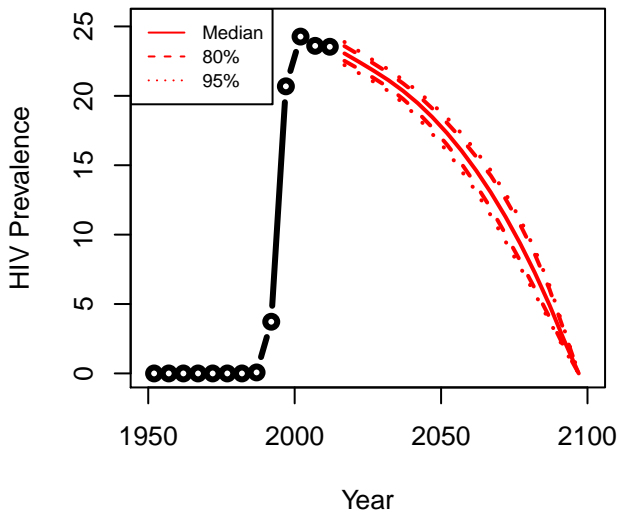

**Liberia**

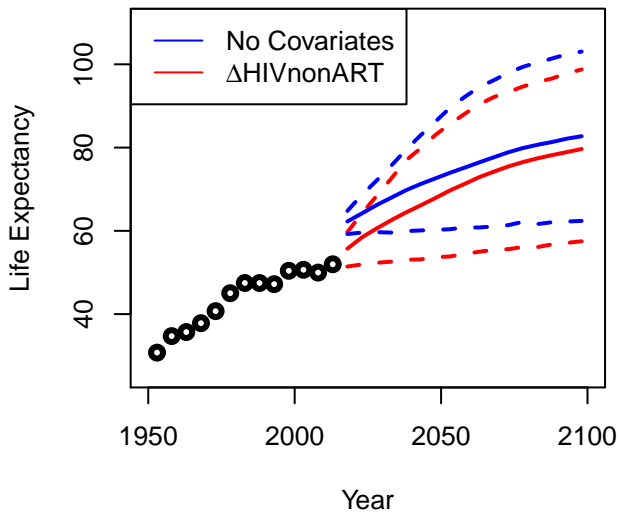

**Liberia**

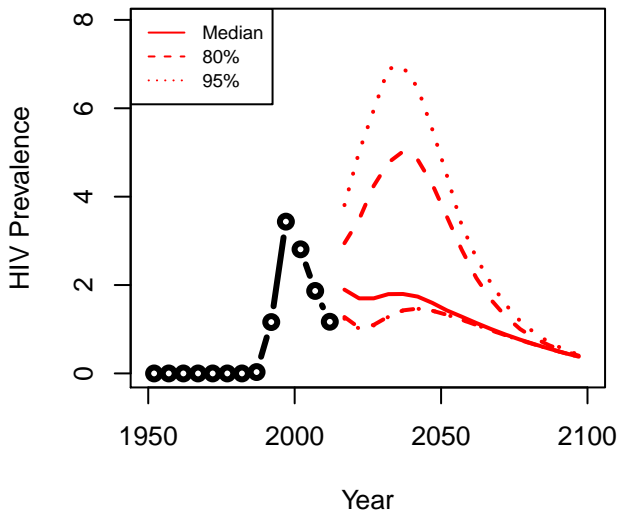

**Malawi**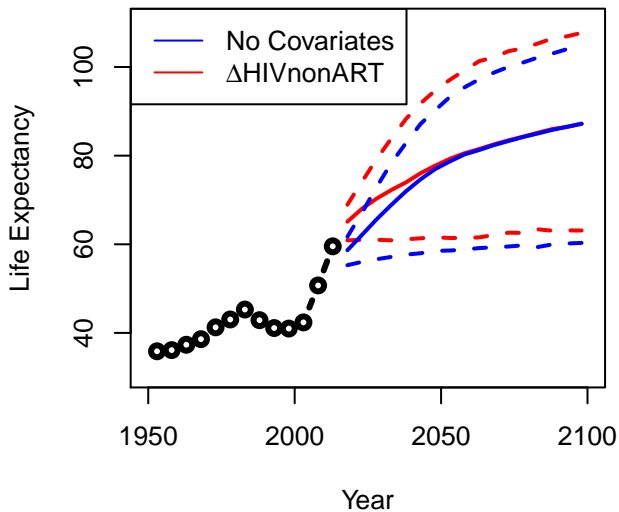**Malawi**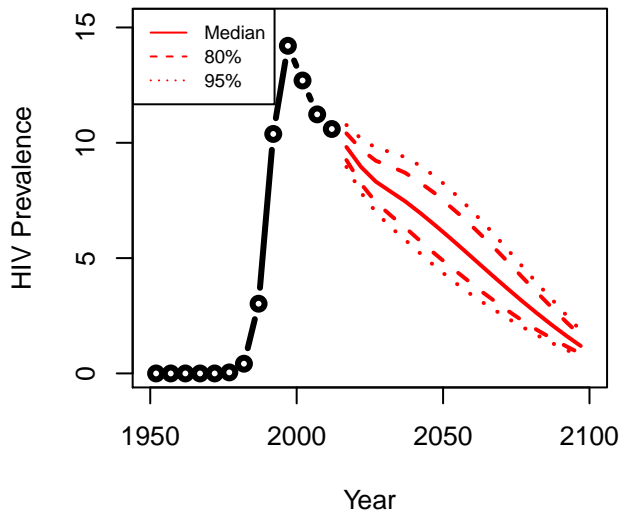**Mali**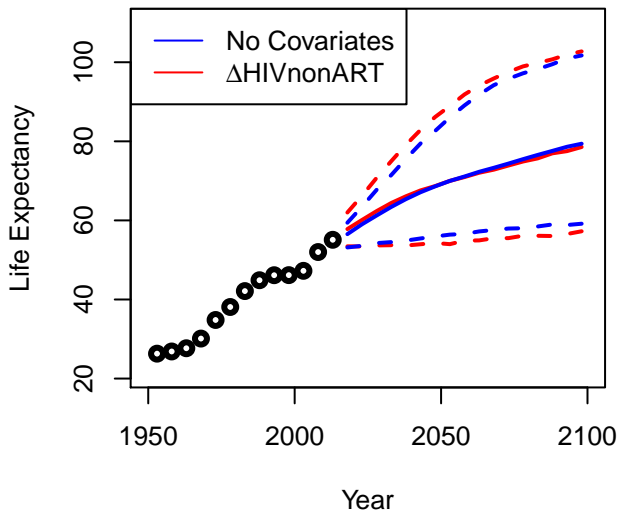**Mali**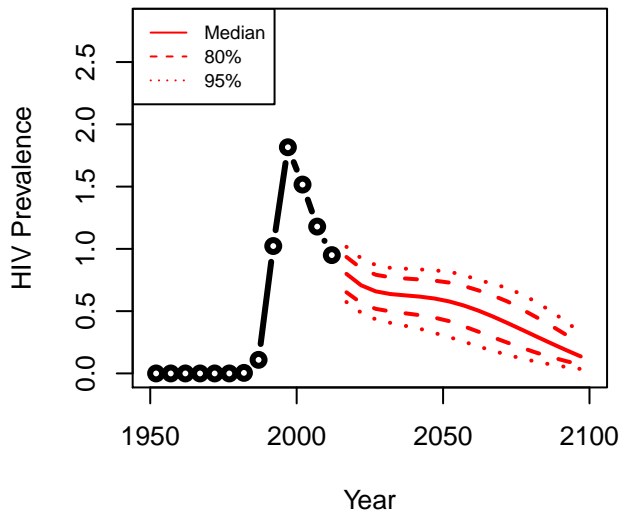

### Mozambique

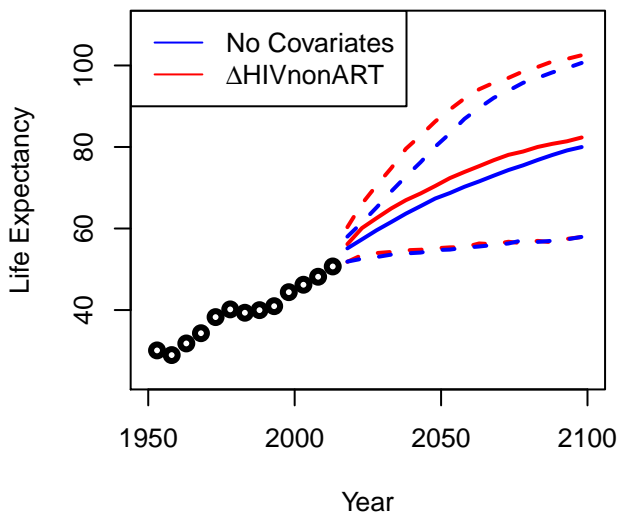

### Mozambique

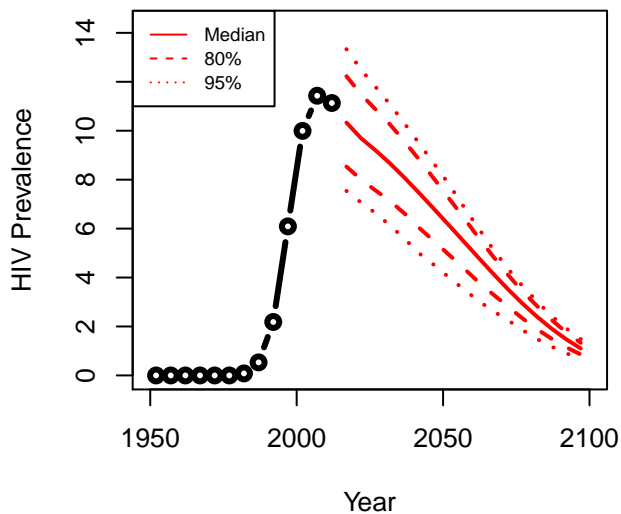

### Namibia

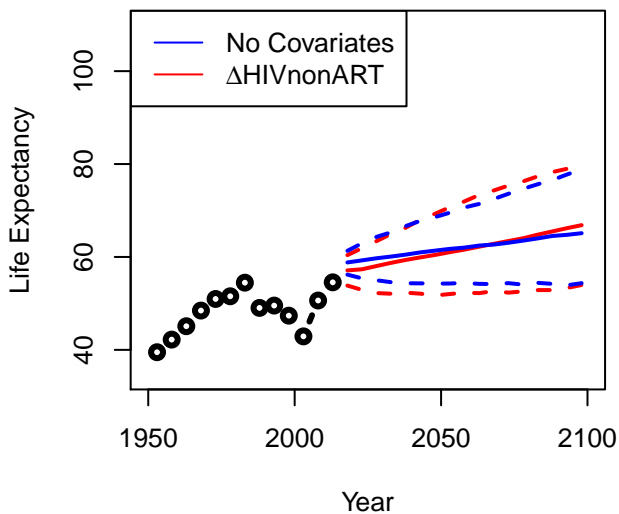

### Namibia

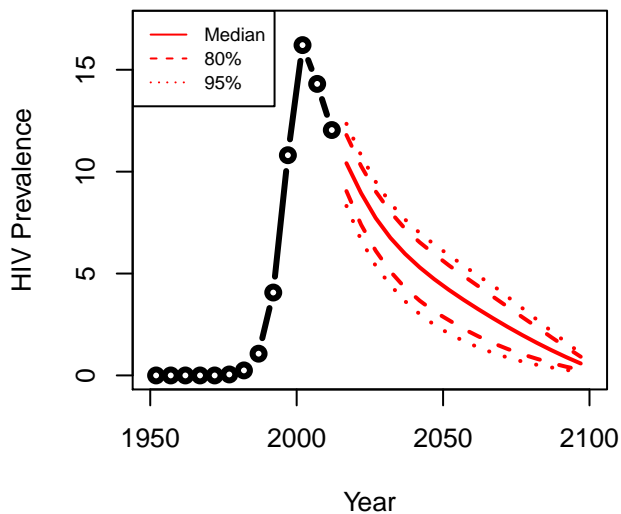

### Nigeria

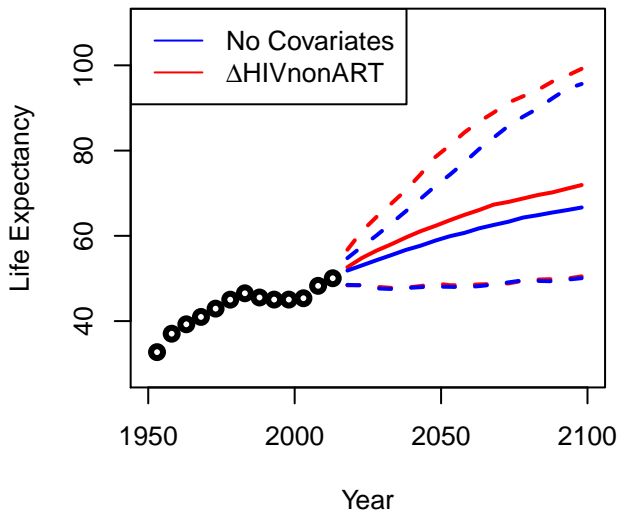

### Nigeria

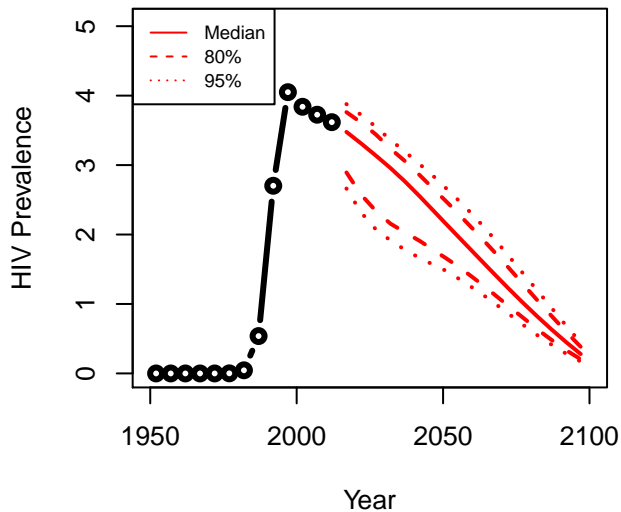

### Rwanda

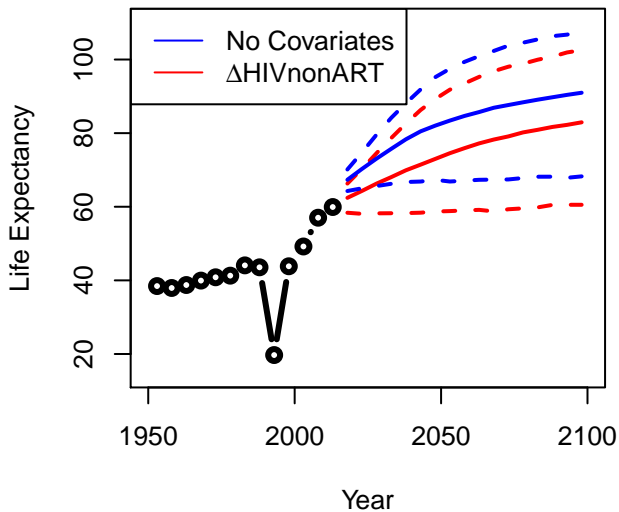

### Rwanda

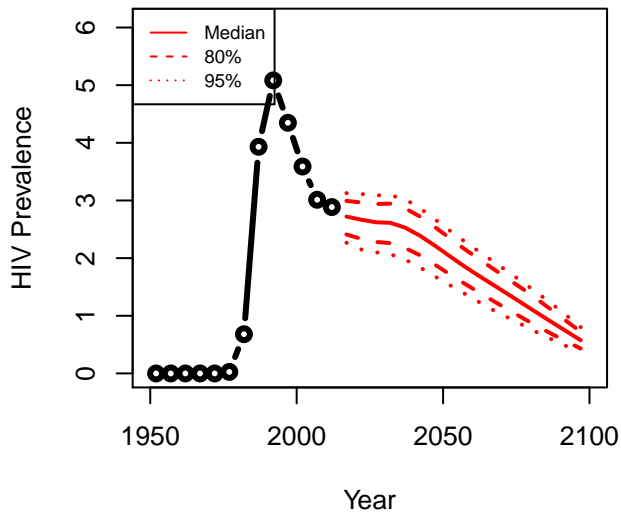



### Sierra Leone

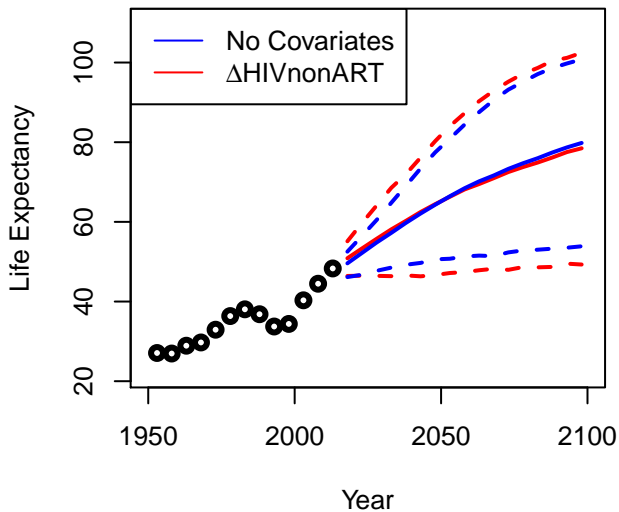

### Sierra Leone

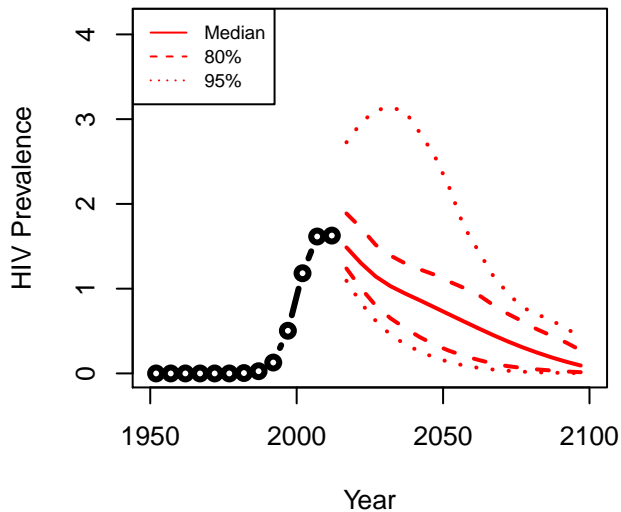

### South Africa

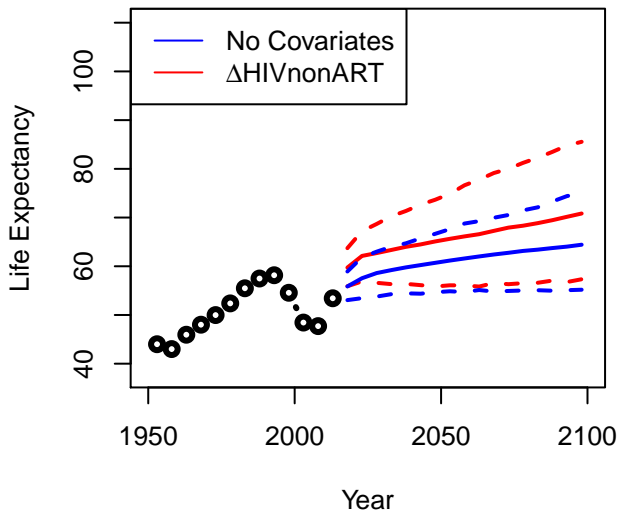

### South Africa

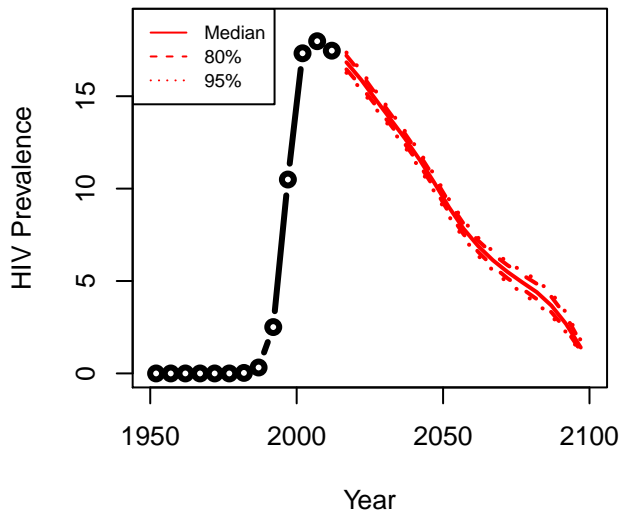

**Swaziland**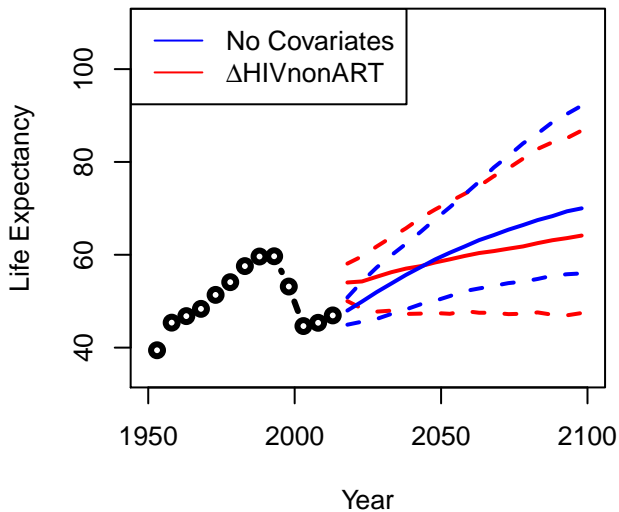**Swaziland**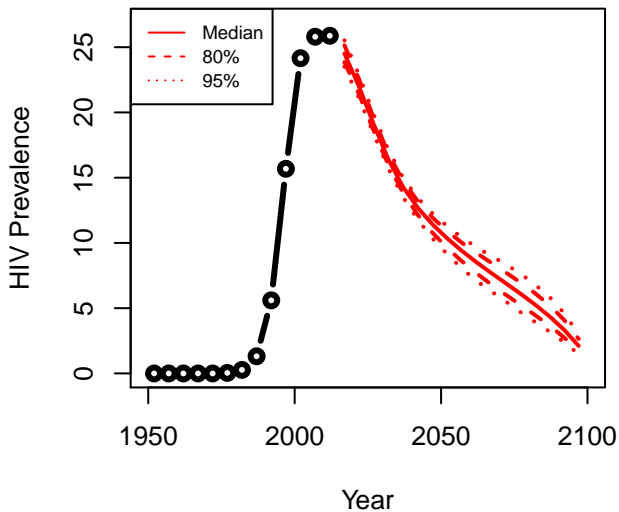**Togo**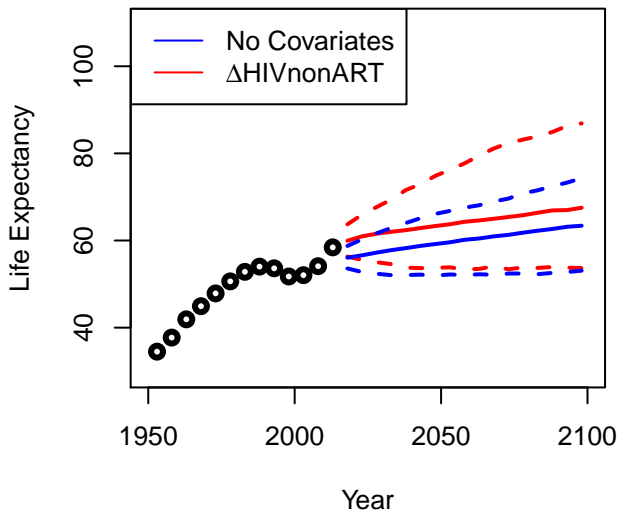**Togo**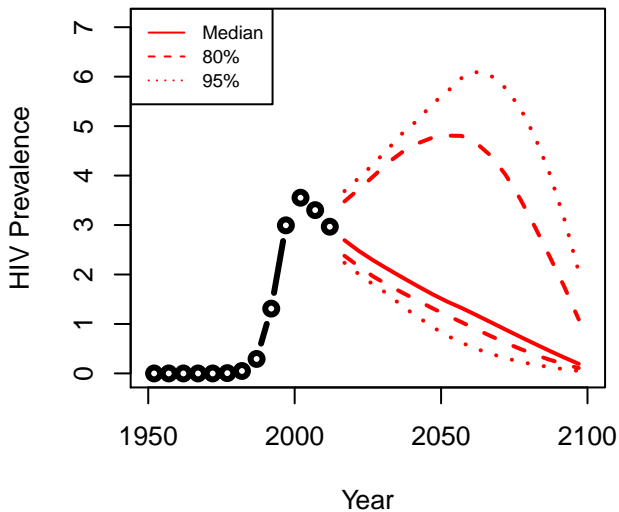

### Uganda

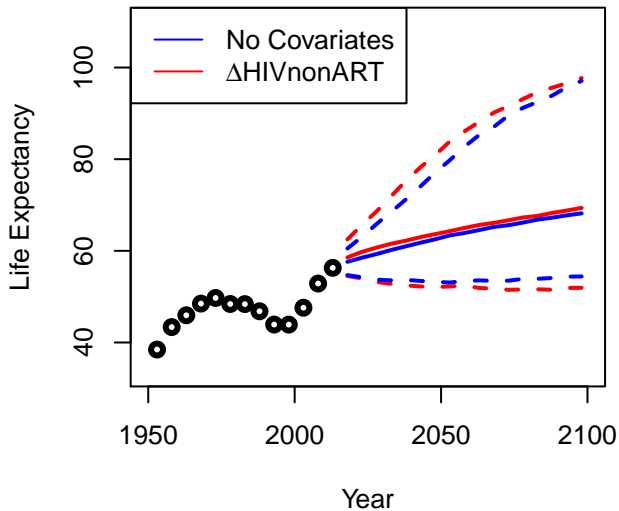

### Uganda

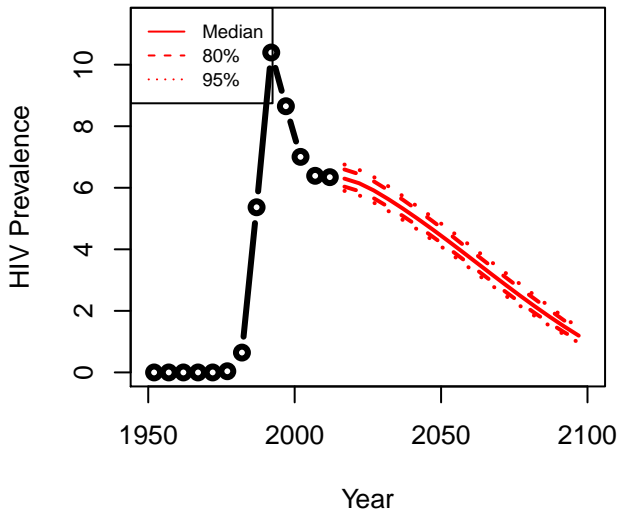

### United Republic of Tanzania

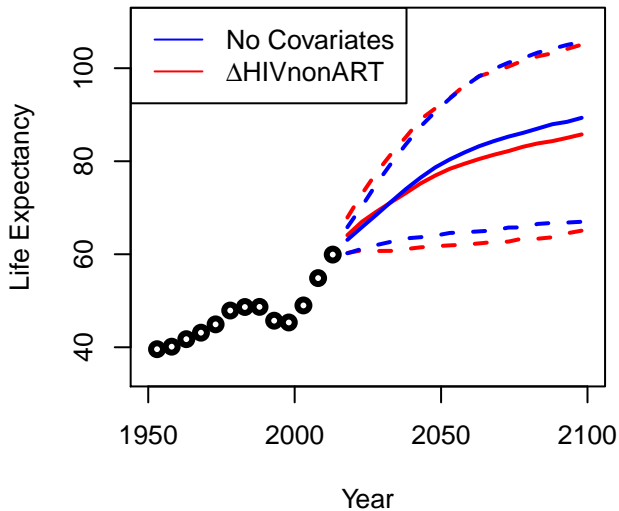

### United Republic of Tanzania

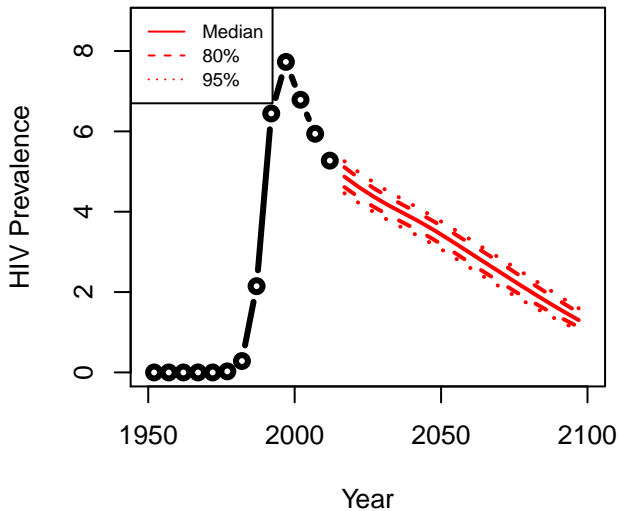

### Zambia

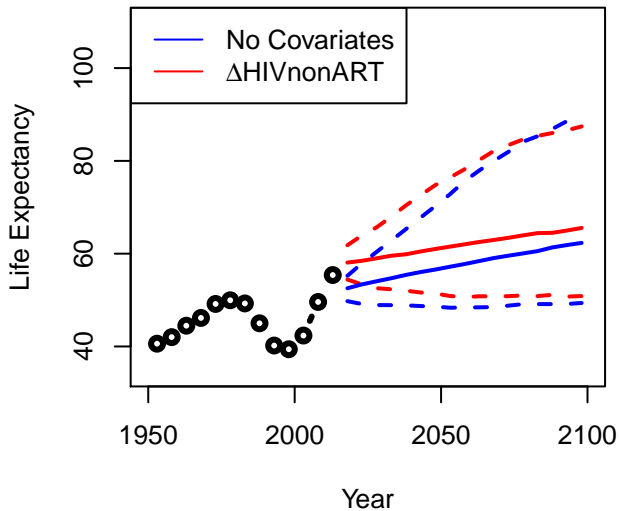

### Zambia

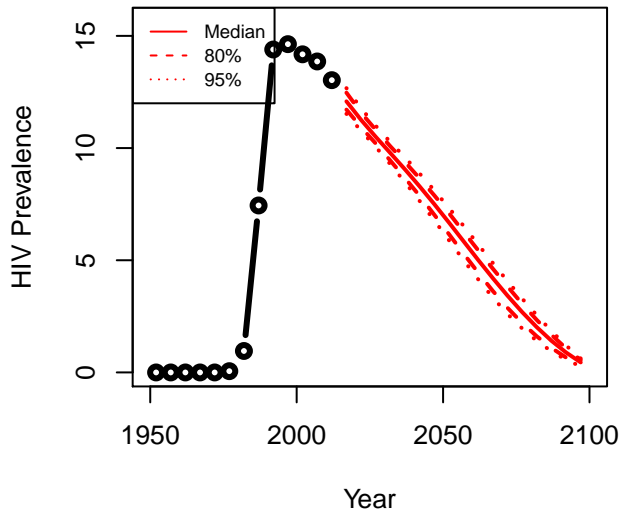

### Zimbabwe

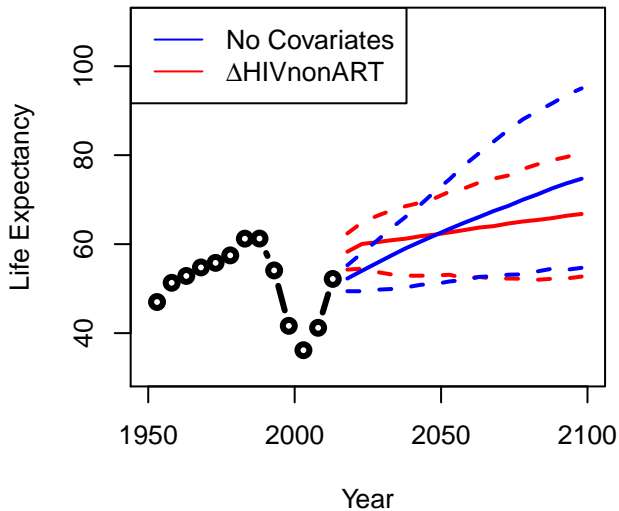

### Zimbabwe

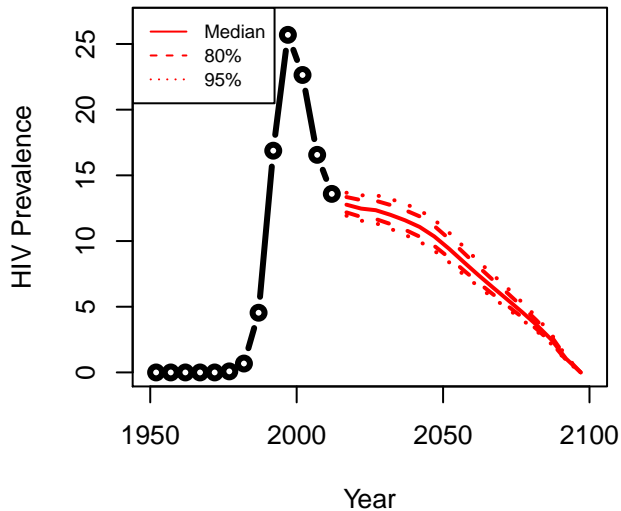

Supplement: Supplementary file 2 [file AppendixUNEPPHIVnonARTMale.pdf]
